# Supplementary material for: Attention to Trajectory: Trajectory-Aware Open-Vocabulary Tracking
Source: arXiv:2503.08145 source file (2025-03-11)
Supplement: Supplementary file 1 [file X_suppl.tex]

\clearpage
\setcounter{page}{1}
\setcounter{equation}{0}
\maketitlesupplementary

In this supplementary material, we provide further elaboration on our proposed method \textbf{TRACT}. Specially, \textbf{S1} delineates the specific structures of the five feature fusion mechanisms in the proposed \textbf{TraCLIP}. Within \textbf{S2}, we present details of the loss function deployed for the training of TRACT. In \textbf{S3} we provide details of the parameter settings used in our experiments. \textbf{S4} delineates the visualization and detailed analysis of the detection density problem. We demonstrates the visualization results of TRACT in \textbf{S5}. Lastly, \textbf{S6} details the meticulously crafted 1203 category descriptions we used.

\section*{S1 Feature Fusion Mechanisms}

In Sec.~\ref{sec:traclip}, we compare five different feature fusion mechanisms, as shown in Fig.~\ref{fig:fusion}. They all take $N$ features $\{ f\}_{i=1}^N$ belonging to the same trajectory sample as input, and adopt different feature fusion mechanisms to integrate discrete features.

\noindent
\textbf{Average-based fusion.} The simplest way is to average the features (see Fig.~\ref{fig:fusion} (a)), which has the advantages of being parameter-free and highly efficient. The fusion process is formulated as follows:
\begin{equation}
    {\breve \bf f} = {\tt Avg}(\{ f\}_{i=1}^N)
\end{equation}
where ${\breve \bf f}$ represents the output trajectory feature, and ${\tt Avg}(\cdot)$ represents the average function along the sequence dimension.

\noindent
\textbf{Attention-based fusion.} As depicted in Fig.~\ref{fig:fusion} (b), the attention-based fusion strategy employs a self-attention module to achieve information interaction within the trajectory. In specific, it takes the input features $\{ f\}_{i=1}^N$ as a sequential data, and fuse them as follows:
\begin{equation}
    {\breve \bf f} = {\tt Avg}({\tt SA}(\{ f\}_{i=1}^N))
\end{equation}
where ${\tt SA}(\cdot)$ denotes self-attention module.

\noindent
\textbf{Self-based fusion.} The self-based fusion mechanism, which we employ in the TFA strategy, is similar to the attention-based one (see Fig.~\ref{fig:fusion} (c)). In addition to the self-attention module, it also utilizes an MLP for further information interaction, as follows:
\begin{equation}
    {\breve \bf f} = {\tt Avg}({\tt MLP}({\tt SA}(\{ f\}_{i=1}^N)))
\end{equation}
where ${\tt MLP}(\cdot)$ is the multi-layer Perceptron module. Experimental results show that this approach achieves the best performance.

\noindent
\textbf{Cross-based fusion.} The fundamental concept of cross-based fusion involves sequentially feed $N$ features as $K/V$ into a cross-attention module, with each step's outcome serving as the subsequent fusion's $Q$ (see Fig.~\ref{fig:fusion} (d)). In specific, the fused trajectory feature ${\dot f}_i$ up to the $i^{th}$ target in the trajectory is formulated as follows:
\begin{equation}
    {\dot f}_i = {\tt CA}({\dot f}_{i-1}, f_i) \qquad i>1
\end{equation}
where ${\tt CA}({\bf x}, {\bf y})$ denotes the cross-attention with ${\bf x}$ as query and ${\bf y}$ as key and value. For the first feature, we set ${\dot f}_1 = f_1$. Finally, cross-based fusion module outputs the trajectory feature ${\breve \bf f} = {\dot f}_N$.

\begin{figure}[t]
 \centering
 \includegraphics[width=0.99\linewidth]{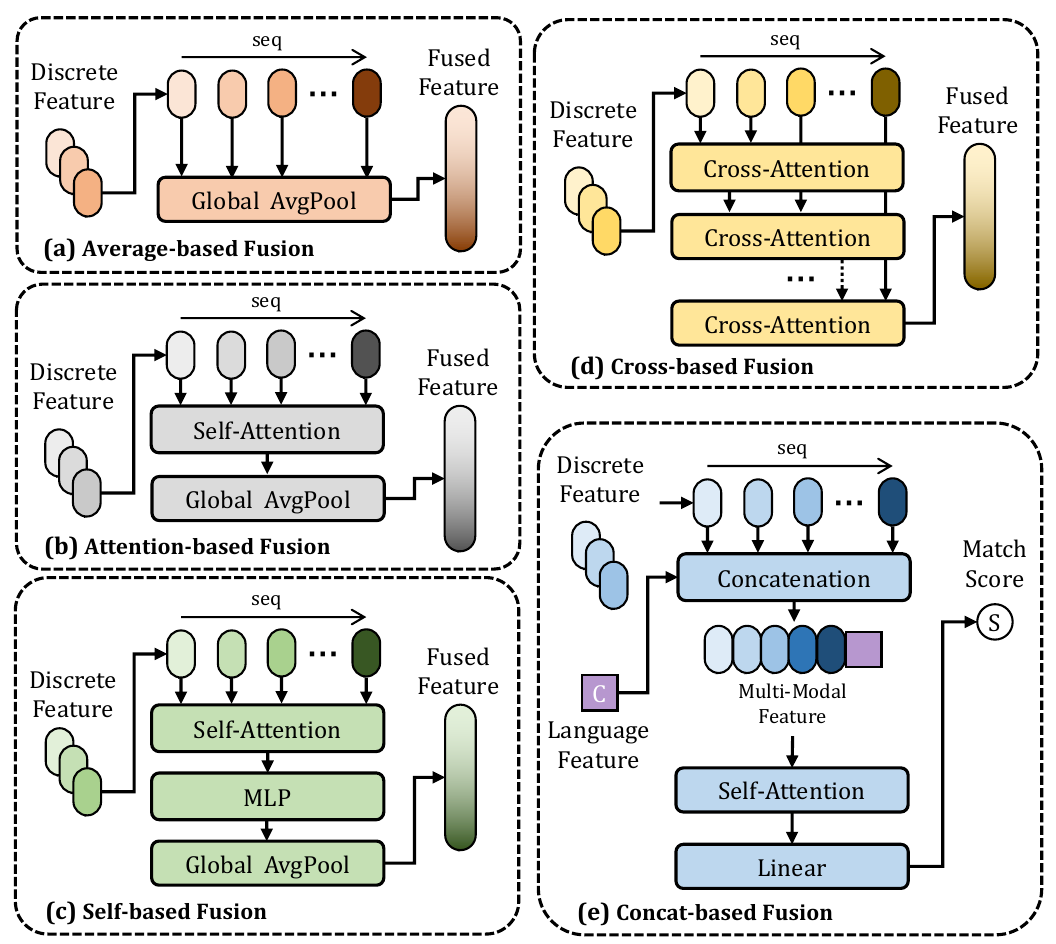}
 %\vspace{-1em}
 \caption{Detailed architectures of the studied 5 fusion mechanisms, \ie, average-based fusion (a), attention-based fusion (b), self-based fusion (c), cross-based fusion (d), and concatenation-based fusion (e).}
 \label{fig:fusion}
 % \vspace{-5mm}
\end{figure}

\noindent
\textbf{Concatenation-based fusion.} As shown in Fig.~\ref{fig:fusion}, the concatenation-based fusion strategy first concatenates $N$ discrete visual features $\{f\}_{i=1}^N \in {\mathbb R}^{N \times m}$ with the language feature of a target category $c \in {\mathbb R}^{1 \times m}$ along the sequence dimension, resulting in a unified multi-modal feature tensor ${\dot f} = {\tt Concat}(f_i, f_2, ..., f_N, c) \in {\mathbb R}^{(N+1) \times m}$. It then uses a self-attention module and two linear projection layers to obtain the similarity score for the corresponding category, as follws:
\begin{equation}
    s = {\tt FC}({\tt Pool}({\tt SA}({\tt Concat}(f_i, f_2, ..., f_N, c))))
\end{equation}
where ${\tt Pool}(\cdot)$ is a projection layer used for internal information interaction, while ${\tt FC}(\cdot)$ is a projection layer used to obtain the score. Please note, unlike previous fusion strategies, the concatenation-based fusion strategy directly produces classification scores for each category.

\begin{figure}[t]
 \centering
 \includegraphics[width=0.99\linewidth]{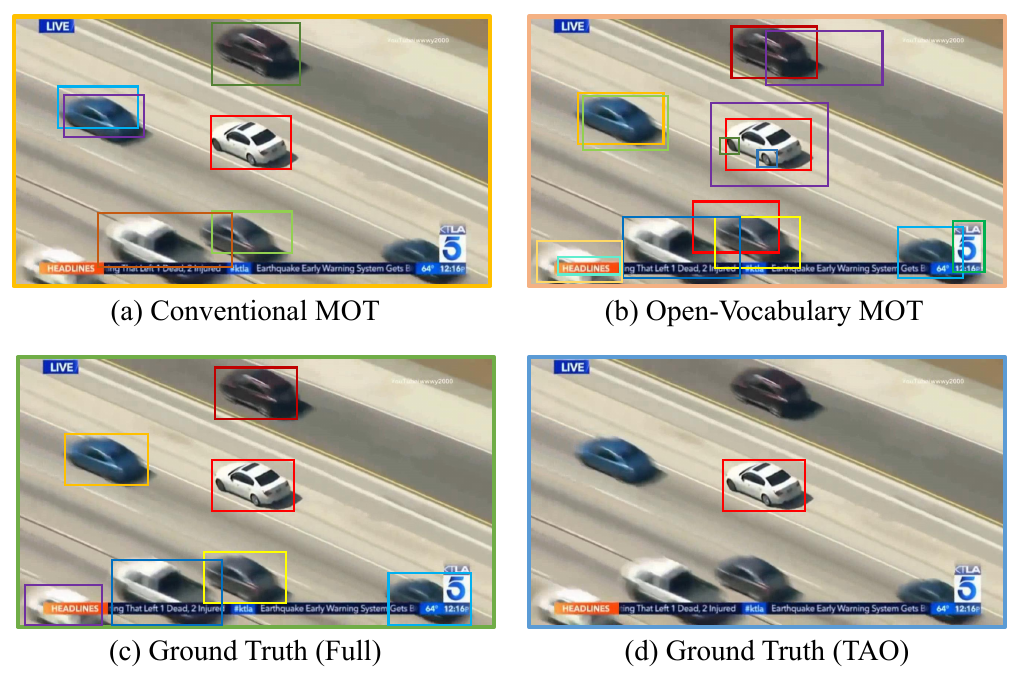}
 %\vspace{-1em}
 \caption{A visual comparison between Conventional MOT detections (a), OV-MOT detections (b), the complete GT annotations (c), and the GT annotations provided by TAO (d). It clearly reveals two points: first, the detection density of OV-MOT is significantly higher than that of Conventional MOT, and second, the GT annotations provided by TAO are incomplete.}
 \label{fig:discussion}
 % \vspace{-5mm}
\end{figure}

\section*{S2 Detailed Training Strategy}

The training of TRACT is divided into two main parts: training for the trajectory-enhanced association step and training for the trajectory-assisted classification step. For the former, we use the method proposed in MASA~\cite{li2024matching}, leveraging SAM~\cite{kirillov2023segment} to enable training on unlabeled image data. For the latter, we train using a contrastive learning loss.

% Contrastive loss is a popular metric learning approach aimed at learning an embedding space by reducing the distance between similar samples and increasing the distance between dissimilar samples. This technique is widely used in tasks that require measuring sample similarity, such as face recognition and image retrieval.

In contrastive learning, given a pair of samples \((x_i, x_j)\), we assign a label \(y_{ij}\) to indicate whether the two samples belong to the same class. If \(y_{ij} = 1\), then \(x_i\) and \(x_j\) are similar (a positive sample pair), whereas if \(y_{ij} = 0\), they are dissimilar (a negative sample pair). The contrastive loss function is defined as follows:
\begin{equation}
    \begin{split}
        \mathcal{L}(x_i, x_j) = &\frac{1}{2} \Big( y_{ij} \cdot D(x_i, x_j)^2 + \\
        &(1 - y_{ij}) \cdot \max \big( 0, m - D(x_i, x_j) \big)^2 \Big)
    \end{split}
\end{equation}
where \(D(x_i, x_j)\) represents the distance between samples \(x_i\) and \(x_j\), which is often measured using Euclidean or cosine distance. The term \(m\) is a margin parameter that enforces a minimum distance between dissimilar pairs. For similar pairs \((y_{ij} = 1)\), the loss \(\frac{1}{2} D(x_i, x_j)^2\) encourages a smaller distance, effectively pulling similar pairs closer together. For dissimilar pairs \((y_{ij} = 0)\), the loss \(\frac{1}{2} \max(0, m - D(x_i, x_j))^2\) promotes a distance of at least \(m\), pushing these pairs farther apart.

The objective of contrastive loss is to learn an embedding space in which similar samples are clustered closely, while dissimilar samples are separated by a clear margin, thereby creating a well-defined separation in the embedding space.

\begin{figure}[t]
    % \vspace{-1em}
    \centering
    \includegraphics[width=0.8\linewidth]{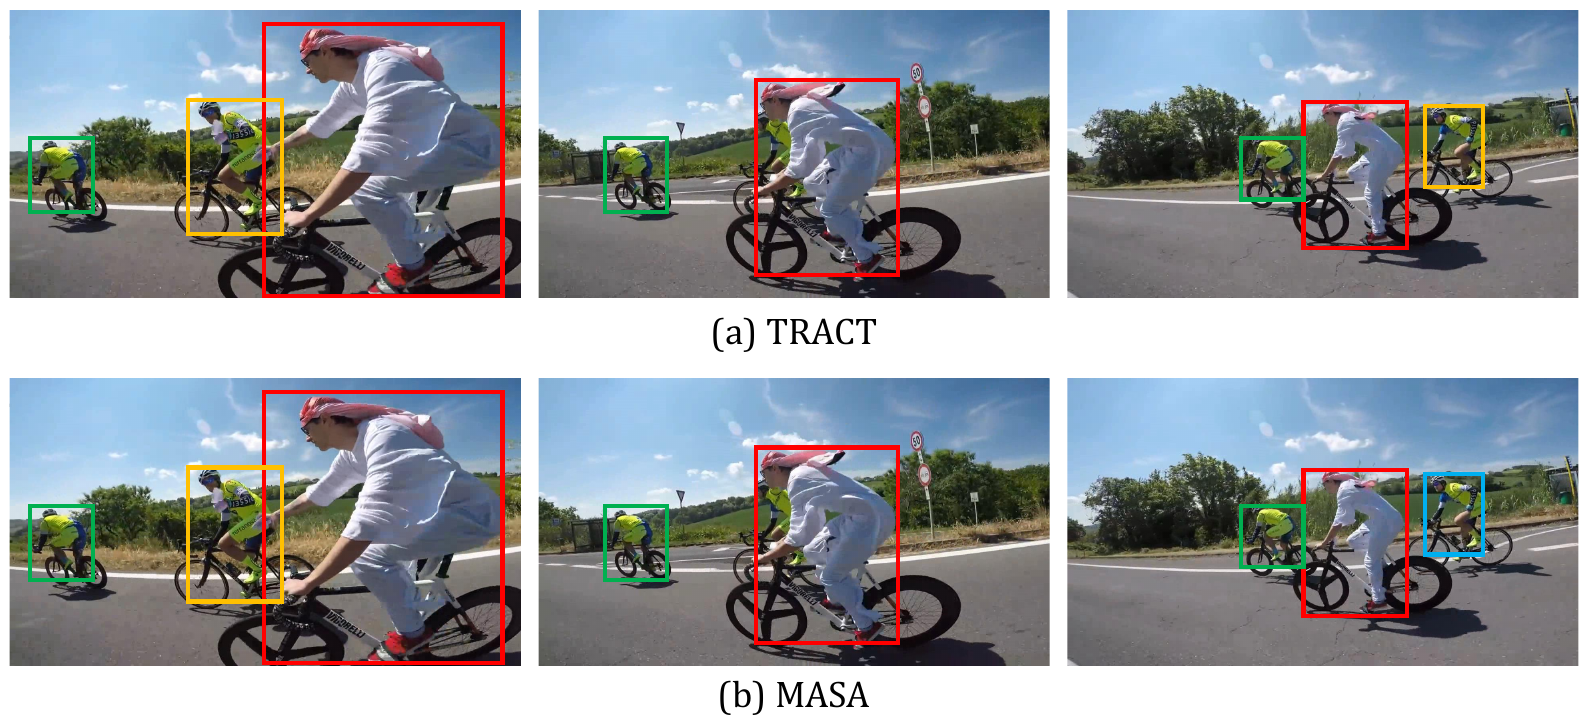}
    \vspace{-1em}
    \caption{Performance under occlusion condition.}
    \label{fig:occlusion}
    \vspace{-5mm}
\end{figure}

\section*{S3 Experiment Settings}

In Sec.~\ref{sec:setup}, we introduced some of the parameter settings used in our experiments. Due to space limitations, we provide a more detailed description here. Specially, during inference, we set the matching threshold $\tau_{\rm match} = 0.4$. Additionally, there are two critical parameters, $\tau_{\rm high}$ and $\tau_{\rm low}$, used in the association process. Since they are closely related to the score range provided by the detection results, we set different values for these parameters depending on the detector used. Specifically, when using ViLD~\cite{gu2021open} and YOLO-World~\cite{cheng2024yolo} as the detector, we set $\tau_{\rm high} = 0.3$ and $\tau_{\rm low} = 0.1$. While using RegionCLIP~\cite{zhong2022regionclip}, since the confidence score consists of two components, values greater than 1 can occur. To adapt this for tracking purposes, we divide the confidence score by 10, which in turn requires adjusting $\tau_{\rm high}$ and $\tau_{\rm low}$ to 0.01 and 0.005, respectively.

\section*{S4 Detection Density Visualization}

As analyzed in Sec.~\ref{sec:discussion}, one reason why OV-MOT is challenging, in addition to the primary classification difficulties, lies in the association difficulty arising from the dense detection results. As illustrated in Fig.~\ref{fig:discussion}, the detection density in OV-MOT (typically evaluated with the TETA metric~\cite{li2022tracking}) is significantly higher than in conventional MOT (evaluated with the HOTA metric). We attribute this to incomplete annotation in the TAO dataset, which includes over 800 categories but lacks exhaustive annotations for most of them. This issue intensifies in the OV-MOT setting, where the TETA metric employs a strategy that does \textit{not} penalize predictions unmatchable to ground-truth annotations. While this approach mitigates the issue of incomplete annotations, it also lessens penalties for numerous false positives. Consequently, detectors often lower detection thresholds to improve tracking of rare categories, resulting in dense and potentially low-quality detection outputs that complicate association further. In summary, we argue that the main challenges in OV-MOT stem from data and evaluation conventions. We hope the OV-MOT community will prioritize addressing these fundamental issues over refining surface-level solutions.

\section*{S5 Tracking Results Visualization}

A key advantage of using trajectory information is the improved tracking performance under occlusion conditions. We demonstrate the visualization of this scenario in Fig.~\ref{fig:occlusion}. We can observe that, compared to MASA, TRACT better maintains the stability of target ids after detection loss.

\section*{S6 Descriptions with Attributes}

OV-TAO use the 1203 categories defined in LVIS dataset, including 866 base classes and 337 novel classes. In TraCLIP, we propose the Trajectory Semantic Enrichment (\textbf{TSE}) strategy to enhance language features using category descriptions. In order to able understanding of TSE, below we present each category description:

\noindent
\textbf{aerosol\_can:}\textit{ cylindrical container with a spray nozzle on top.}

\noindent
\textbf{air\_conditioner:}\textit{ boxy unit with vents for cooling air.}

\noindent
\textbf{airplane:}\textit{ streamlined body with wings and tail.}

\noindent
\textbf{alarm\_clock:}\textit{ small rectangular device with a face and hands.}

\noindent
\textbf{alcohol:}\textit{ clear or amber liquid in a bottle.}

\noindent
\textbf{alligator:}\textit{ thick, scaly body with a long snout.}

\noindent
\textbf{almond:}\textit{ oval-shaped nut with a brown skin.}

\noindent
\textbf{ambulance:}\textit{ white vehicle with a red cross and siren.}

\noindent
\textbf{amplifier:}\textit{ boxy device with knobs and speaker connections.}

\noindent
\textbf{anklet:}\textit{ decorative band worn around the ankle.}

\noindent
\textbf{antenna:}\textit{ long, thin rod extending from a device.}

\noindent
\textbf{apple:}\textit{ round fruit with a smooth skin.}

\noindent
\textbf{applesauce:}\textit{ smooth, chunky puree in a jar.}

\noindent
\textbf{apricot:}\textit{ small, orange fruit with a fuzzy skin.}

\noindent
\textbf{apron:}\textit{ cloth garment worn over the front of clothes.}

\noindent
\textbf{aquarium:}\textit{ glass tank filled with water and fish.}

\noindent
\textbf{arctic\_(type\_of\_shoe):}\textit{ insulated boot with a thick sole.}

\noindent
\textbf{armband:}\textit{ fabric band worn on the arm, often colorful.}

\noindent
\textbf{armchair:}\textit{ soft chair with armrests and a cushioned seat.}

\noindent
\textbf{armoire:}\textit{ tall, freestanding cabinet with doors.}

\noindent
\textbf{armor:}\textit{ protective metal covering for the body.}

\noindent
\textbf{artichoke:}\textit{ green, spiky vegetable shaped like a flower.}

\noindent
\textbf{trash\_can:}\textit{ cylindrical container for waste with a lid.}

\noindent
\textbf{ashtray:}\textit{ shallow dish for holding cigarette ashes.}

\noindent
\textbf{asparagus:}\textit{ long, thin green vegetable with a pointed tip.}

\noindent
\textbf{atomizer:}\textit{ small bottle with a spray nozzle for perfumes.}

\noindent
\textbf{avocado:}\textit{ green, pear-shaped fruit with a rough skin.}

\noindent
\textbf{award:}\textit{ decorative object, often in the shape of a trophy.}

\noindent
\textbf{awning:}\textit{ fabric canopy extending over a doorway.}

\noindent
\textbf{ax:}\textit{ heavy tool with a sharp blade for chopping.}

\noindent
\textbf{baboon:}\textit{ large primate with a long face and colorful rear.}

\noindent
\textbf{baby\_buggy:}\textit{ wheeled carriage for transporting infants.}

\noindent
\textbf{basketball\_backboard:}\textit{ large, flat surface with a hoop attached.}

\noindent
\textbf{backpack:}\textit{ fabric bag with straps worn on the back.}

\noindent
\textbf{handbag:}\textit{ small purse carried by hand or on the shoulder.}

\noindent
\textbf{suitcase:}\textit{ hard or soft case for carrying clothes.}

\noindent
\textbf{bagel:}\textit{ round bread with a hole in the center.}

\noindent
\textbf{bagpipe:}\textit{ musical instrument with pipes and a bag.}

\noindent
\textbf{baguet:}\textit{ long, thin loaf of french bread.}

\noindent
\textbf{bait:}\textit{ lure, often in the form of small fish or worms.}

\noindent
\textbf{ball:}\textit{ round object used in various games.}

\noindent
\textbf{ballet\_skirt:}\textit{ flowy, short skirt often made of tulle.}

\noindent
\textbf{balloon:}\textit{ inflatable round object made of rubber or plastic.}

\noindent
\textbf{bamboo:}\textit{ tall, slender grass with hollow stems.}

\noindent
\textbf{banana:}\textit{ curved, yellow fruit with a soft interior.}

\noindent
\textbf{band\_aid:}\textit{ small adhesive strip with a sterile pad.}

\noindent
\textbf{bandage:}\textit{ cloth strip used to cover wounds.}

\noindent
\textbf{bandanna:}\textit{ square piece of cloth tied around the head or neck.}

\noindent
\textbf{banjo:}\textit{ string instrument with a circular body and neck.}

\noindent
\textbf{banner:}\textit{ large piece of cloth with words or images displayed.}

\noindent
\textbf{barbell:}\textit{ long metal rod with weights on both ends.}

\noindent
\textbf{barge:}\textit{ flat-bottomed boat used for transporting goods.}

\noindent
\textbf{barrel:}\textit{ round container used for storage, often made of wood.}

\noindent
\textbf{barrette:}\textit{ hair clip used to hold hair in place.}

\noindent
\textbf{barrow:}\textit{ wheelbarrow with a large, open bed.}

\noindent
\textbf{baseball\_base:}\textit{ square rubber pad used in baseball fields.}

\noindent
\textbf{baseball:}\textit{ round ball with a leather cover and stitching.}

\noindent
\textbf{baseball\_bat:}\textit{ long, cylindrical piece of wood or metal.}

\noindent
\textbf{baseball\_cap:}\textit{ soft cap with a curved brim.}

\noindent
\textbf{baseball\_glove:}\textit{ leather glove designed for catching baseballs.}

\noindent
\textbf{basket:}\textit{ woven container used for carrying items.}

\noindent
\textbf{basketball:}\textit{ round ball with a textured surface.}

\noindent
\textbf{bass\_horn:}\textit{ large brass instrument with a wide bell.}

\noindent
\textbf{bat\_(animal):}\textit{ winged mammal with a fur-covered body.}

\noindent
\textbf{bath\_mat:}\textit{ soft, absorbent mat placed outside a bathtub.}

\noindent
\textbf{bath\_towel:}\textit{ large, absorbent cloth for drying off.}

\noindent
\textbf{bathrobe:}\textit{ loose-fitting garment worn after bathing.}

\noindent
\textbf{bathtub:}\textit{ enclosed basin for bathing, often with a faucet.}

\noindent
\textbf{batter\_(food):}\textit{ thick mixture used for baking or frying.}

\noindent
\textbf{battery:}\textit{ rectangular device that stores electrical energy.}

\noindent
\textbf{beachball:}\textit{ large, inflatable ball for playing at the beach.}

\noindent
\textbf{bead:}\textit{ small, round object often used in jewelry making.}

\noindent
\textbf{bean\_curd:}\textit{ soft, pale food made from soybeans.}

\noindent
\textbf{beanbag:}\textit{ soft, cushioned bag filled with beans or foam.}

\noindent
\textbf{beanie:}\textit{ close-fitting, knitted hat.}

\noindent
\textbf{bear:}\textit{ large, furry mammal with a broad body.}

\noindent
\textbf{bed:}\textit{ rectangular piece of furniture for sleeping.}

\noindent
\textbf{bedpan:}\textit{ shallow container for bodily waste.}

\noindent
\textbf{bedspread:}\textit{ decorative covering for a bed.}

\noindent
\textbf{cow:}\textit{ large farm animal with a sturdy body and udder.}

\noindent
\textbf{beef\_(food):}\textit{ red meat cut from a cow.}

\noindent
\textbf{beeper:}\textit{ small device that emits sound or alerts.}

\noindent
\textbf{beer\_bottle:}\textit{ tall glass container for beer.}

\noindent
\textbf{beer\_can:}\textit{ metal container for beer, often cylindrical.}

\noindent
\textbf{beetle:}\textit{ small, hard-bodied insect with antennae.}

\noindent
\textbf{bell:}\textit{ round object that makes a ringing sound.}

\noindent
\textbf{bell\_pepper:}\textit{ colorful vegetable with a bell shape.}

\noindent
\textbf{belt:}\textit{ flexible band worn around the waist.}

\noindent
\textbf{belt\_buckle:}\textit{ decorative fastener for a belt.}

\noindent
\textbf{bench:}\textit{ long seat with no backrest.}

\noindent
\textbf{beret:}\textit{ soft, round hat often worn tilted.}

\noindent
\textbf{bib:}\textit{ cloth or plastic garment worn to protect clothing.}

\noindent
\textbf{bible:}\textit{ bound book with a leather or cloth cover.}

\noindent
\textbf{bicycle:}\textit{ two-wheeled vehicle powered by pedaling.}

\noindent
\textbf{visor:}\textit{ brimmed headwear that shields the eyes.}

\noindent
\textbf{billboard:}\textit{ large outdoor advertising structure.}

\noindent
\textbf{binder:}\textit{ cover with rings for holding loose papers.}

\noindent
\textbf{binoculars:}\textit{ two-tube device for magnifying distant objects.}

\noindent
\textbf{bird:}\textit{ small, feathered animal with wings.}

\noindent
\textbf{birdfeeder:}\textit{ container designed to hold birdseed.}

\noindent
\textbf{birdbath:}\textit{ shallow basin for birds to bathe in.}

\noindent
\textbf{birdcage:}\textit{ enclosed space with bars for housing birds.}

\noindent
\textbf{birdhouse:}\textit{ small wooden structure for nesting birds.}

\noindent
\textbf{birthday\_cake:}\textit{ decorated cake typically with candles on top.}

\noindent
\textbf{birthday\_card:}\textit{ greeting card designed for birthday wishes.}

\noindent
\textbf{pirate\_flag:}\textit{ black flag with a skull and crossbones design.}

\noindent
\textbf{black\_sheep:}\textit{ sheep with black wool, often symbolizing uniqueness.}

\noindent
\textbf{blackberry:}\textit{ dark purple fruit with small, edible seeds.}

\noindent
\textbf{blackboard:}\textit{ dark surface for writing with chalk.}

\noindent
\textbf{blanket:}\textit{ soft covering for warmth, often made of fabric.}

\noindent
\textbf{blazer:}\textit{ tailored jacket, typically with a single-breasted front.}

\noindent
\textbf{blender:}\textit{ kitchen appliance with a jar and blades for mixing.}

\noindent
\textbf{blimp:}\textit{ large, inflatable airship with a rounded shape.}

\noindent
\textbf{blinker:}\textit{ light signal on a vehicle indicating turns.}

\noindent
\textbf{blouse:}\textit{ women’s garment that is loose-fitting and stylish.}

\noindent
\textbf{blueberry:}\textit{ small, round fruit that is blue or purple.}

\noindent
\textbf{gameboard:}\textit{ flat surface marked for playing games.}

\noindent
\textbf{boat:}\textit{ watercraft designed for navigation on water.}

\noindent
\textbf{bob:}\textit{ short haircut that is typically straight around the head.}

\noindent
\textbf{bobbin:}\textit{ small spool for holding thread or yarn.}

\noindent
\textbf{bobby\_pin:}\textit{ hairpin used to hold hair in place.}

\noindent
\textbf{boiled\_egg:}\textit{ egg that has been cooked in boiling water.}

\noindent
\textbf{bolo\_tie:}\textit{ neckwear consisting of a cord with decorative tips.}

\noindent
\textbf{deadbolt:}\textit{ locking mechanism with a solid metal bolt.}

\noindent
\textbf{bolt:}\textit{ metal fastener used for joining objects together.}

\noindent
\textbf{bonnet:}\textit{ soft hat that ties under the chin, often worn by women.}

\noindent
\textbf{book:}\textit{ bound collection of written or printed pages.}

\noindent
\textbf{bookcase:}\textit{ shelved furniture for storing books.}

\noindent
\textbf{booklet:}\textit{ small book with a few pages, often informative.}

\noindent
\textbf{bookmark:}\textit{ strip of paper or fabric used to mark a page.}

\noindent
\textbf{boom\_microphone:}\textit{ long microphone mounted on a boom pole.}

\noindent
\textbf{boot:}\textit{ sturdy footwear that covers the ankle.}

\noindent
\textbf{bottle:}\textit{ container, typically made of glass or plastic, for liquids.}

\noindent
\textbf{bottle\_opener:}\textit{ tool for removing caps from bottles.}

\noindent
\textbf{bouquet:}\textit{ arrangement of flowers, often for gifting.}

\noindent
\textbf{bow\_(weapon):}\textit{ curved weapon used for shooting arrows.}

\noindent
\textbf{bow\_(decorative\_ribbons):}\textit{ fabric ribbon tied in a loop for decoration.}

\noindent
\textbf{bow-tie:}\textit{ necktie shaped like a bow, often worn with formal wear.}

\noindent
\textbf{bowl:}\textit{ round dish used for serving food.}

\noindent
\textbf{pipe\_bowl:}\textit{ part of a pipe where tobacco is placed.}

\noindent
\textbf{bowler\_hat:}\textit{ rounded, hard-brimmed hat often worn by men.}

\noindent
\textbf{bowling\_ball:}\textit{ heavy, spherical ball used in bowling.}

\noindent
\textbf{box:}\textit{ container with a flat base and sides.}

\noindent
\textbf{boxing\_glove:}\textit{ padded glove worn in boxing matches.}

\noindent
\textbf{suspenders:}\textit{ straps worn over the shoulders to hold up trousers.}

\noindent
\textbf{bracelet:}\textit{ decorative band worn around the wrist.}

\noindent
\textbf{brass\_plaque:}\textit{ flat, engraved metal plate for display.}

\noindent
\textbf{brassiere:}\textit{ garment worn to support women’s breasts.}

\noindent
\textbf{bread-bin:}\textit{ container for storing bread to keep it fresh.}

\noindent
\textbf{bread:}\textit{ staple food made from flour and water, often baked.}

\noindent
\textbf{breechcloth:}\textit{ simple garment worn around the waist.}

\noindent
\textbf{bridal\_gown:}\textit{ formal dress worn by a bride during a wedding.}

\noindent
\textbf{briefcase:}\textit{ portable case for carrying documents or laptops.}

\noindent
\textbf{broccoli:}\textit{ green vegetable with a tree-like structure.}

\noindent
\textbf{broach:}\textit{ decorative pin worn on clothing.}

\noindent
\textbf{broom:}\textit{ tool with bristles for sweeping floors.}

\noindent
\textbf{brownie:}\textit{ small, chocolate dessert, often fudgy.}

\noindent
\textbf{brussels\_sprouts:}\textit{ small, round green vegetable resembling cabbage.}

\noindent
\textbf{bubble\_gum:}\textit{ chewy candy that can be blown into bubbles.}

\noindent
\textbf{bucket:}\textit{ container with a handle, typically for carrying liquids.}

\noindent
\textbf{horse\_buggy:}\textit{ small, lightweight carriage pulled by a horse.}

\noindent
\textbf{bull:}\textit{ large, male bovine animal with a sturdy body.}

\noindent
\textbf{bulldog:}\textit{ stocky dog breed with loose skin and a flat face.}

\noindent
\textbf{bulldozer:}\textit{ heavy machinery with a broad blade for pushing earth.}

\noindent
\textbf{bullet\_train:}\textit{ high-speed train designed for rapid travel.}

\noindent
\textbf{bulletin\_board:}\textit{ board for posting notices or announcements.}

\noindent
\textbf{bulletproof\_vest:}\textit{ protective garment designed to resist bullets.}

\noindent
\textbf{bullhorn:}\textit{ loudspeaker used to amplify the voice.}

\noindent
\textbf{bun:}\textit{ round bread roll or a hairstyle with hair pulled back.}

\noindent
\textbf{bunk\_bed:}\textit{ bed with one bed stacked on top of another.}

\noindent
\textbf{buoy:}\textit{ floating marker used to indicate water depths or hazards.}

\noindent
\textbf{burrito:}\textit{ rolled tortilla filled with various ingredients.}

\noindent
\textbf{bus\_(vehicle):}\textit{ large vehicle designed for transporting passengers.}

\noindent
\textbf{business\_card:}\textit{ small card with contact information for professionals.}

\noindent
\textbf{butter:}\textit{ yellow dairy product used for cooking or spreading.}

\noindent
\textbf{butterfly:}\textit{ colorful insect with large, patterned wings.}

\noindent
\textbf{button:}\textit{ small disk used for fastening clothing.}

\noindent
\textbf{cab\_(taxi):}\textit{ vehicle for hire, typically painted in bright colors.}

\noindent
\textbf{cabana:}\textit{ sheltered area often found by a pool or beach.}

\noindent
\textbf{cabin\_car:}\textit{ passenger car used in trains for seating.}

\noindent
\textbf{cabinet:}\textit{ storage unit with shelves and doors, often for kitchen use.}

\noindent
\textbf{locker:}\textit{ enclosed space with a door for storing personal items.}

\noindent
\textbf{cake:}\textit{ sweet baked dessert, often layered and decorated.}

\noindent
\textbf{calculator:}\textit{ electronic device for performing mathematical calculations.}

\noindent
\textbf{calendar:}\textit{ chart displaying days, weeks, and months.}

\noindent
\textbf{calf:}\textit{ young bovine animal.}

\noindent
\textbf{camcorder:}\textit{ portable device for recording video.}

\noindent
\textbf{camel:}\textit{ long-necked animal with a hump, often found in deserts.}

\noindent
\textbf{camera:}\textit{ device for capturing images or video.}

\noindent
\textbf{camera\_lens:}\textit{ optical component used to focus light in cameras.}

\noindent
\textbf{camper\_(vehicle):}\textit{ vehicle designed for living and camping.}

\noindent
\textbf{can:}\textit{ metal container for storing food or beverages.}

\noindent
\textbf{can\_opener:}\textit{ tool for opening metal cans.}

\noindent
\textbf{candle:}\textit{ wax stick with a wick that burns for light.}

\noindent
\textbf{candle\_holder:}\textit{ stand or holder for holding a candle upright.}

\noindent
\textbf{candy\_bar:}\textit{ chocolate-covered confection filled with sweet ingredients.}

\noindent
\textbf{candy\_cane:}\textit{ hard candy shaped like a cane, often striped.}

\noindent
\textbf{walking\_cane:}\textit{ stick used for support while walking.}

\noindent
\textbf{canister:}\textit{ container, typically with a lid, for storing items.}

\noindent
\textbf{canoe:}\textit{ narrow boat propelled by paddling.}

\noindent
\textbf{cantaloup:}\textit{ round, orange-fleshed melon with a netted skin.}

\noindent
\textbf{canteen:}\textit{ container for carrying water or other liquids.}

\noindent
\textbf{cap\_(headwear):}\textit{ soft hat that fits snugly on the head.}

\noindent
\textbf{bottle\_cap:}\textit{ circular cover for sealing a bottle.}

\noindent
\textbf{cape:}\textit{ flowing garment worn over the shoulders.}

\noindent
\textbf{cappuccino:}\textit{ coffee drink made with steamed milk and foam.}

\noindent
\textbf{car\_(automobile):}\textit{ motor vehicle with four wheels for transportation.}

\noindent
\textbf{railcar\_(part\_of\_a\_train):}\textit{ car designed for traveling on railway tracks.}

\noindent
\textbf{elevator\_car:}\textit{ compartment that moves within a building to transport people.}

\noindent
\textbf{car\_battery:}\textit{ rechargeable battery used to power a vehicle.}

\noindent
\textbf{identity\_card:}\textit{ official document that verifies a person’s identity.}

\noindent
\textbf{card:}\textit{ rectangular piece of paper or plastic used for various purposes.}

\noindent
\textbf{cardigan:}\textit{ knitted sweater with an open front and buttons.}

\noindent
\textbf{cargo\_ship:}\textit{ large vessel designed for transporting goods.}

\noindent
\textbf{carnation:}\textit{ flower with frilled petals, often used in bouquets.}

\noindent
\textbf{horse\_carriage:}\textit{ wheeled vehicle pulled by horses for transportation.}

\noindent
\textbf{carrot:}\textit{ long, orange root vegetable with a crunchy texture.}

\noindent
\textbf{tote\_bag:}\textit{ large bag with handles for carrying items.}

\noindent
\textbf{cart:}\textit{ small wheeled vehicle for transporting goods.}

\noindent
\textbf{carton:}\textit{ container made of cardboard for packaging items.}

\noindent
\textbf{cash\_register:}\textit{ machine for recording sales transactions.}

\noindent
\textbf{casserole:}\textit{ dish used for cooking food in the oven.}

\noindent
\textbf{cassette:}\textit{ plastic case containing magnetic tape for audio recording.}

\noindent
\textbf{cast:}\textit{ solid form made to support a broken limb.}

\noindent
\textbf{cat:}\textit{ small domesticated feline known for its agility.}

\noindent
\textbf{cauliflower:}\textit{ white, dense flower vegetable, often used in cooking.}

\noindent
\textbf{cayenne\_(spice):}\textit{ hot, red pepper used as a spice.}

\noindent
\textbf{cd\_player:}\textit{ device for playing compact discs.}

\noindent
\textbf{celery:}\textit{ crisp, green stalk vegetable, often used in salads.}

\noindent
\textbf{cellular\_telephone:}\textit{ portable device for communication over cellular networks.}

\noindent
\textbf{chain\_mail:}\textit{ armor made of interlinked metal rings.}

\noindent
\textbf{chair:}\textit{ seat with a backrest for one person.}

\noindent
\textbf{chaise\_longue:}\textit{ long chair designed for reclining.}

\noindent
\textbf{chalice:}\textit{ decorative cup used for drinking, often in ceremonies.}

\noindent
\textbf{chandelier:}\textit{ ornate lighting fixture hung from the ceiling.}

\noindent
\textbf{chap:}\textit{ informal term for a young man or boy.}

\noindent
\textbf{checkbook:}\textit{ book containing checks for making payments.}

\noindent
\textbf{checkerboard:}\textit{ board with alternating colored squares for playing checkers.}

\noindent
\textbf{cherry:}\textit{ small, round, red or yellow fruit with a pit.}

\noindent
\textbf{chessboard:}\textit{ board with alternating squares for playing chess.}

\noindent
\textbf{chicken\_(animal):}\textit{ domesticated bird raised for meat or eggs.}

\noindent
\textbf{chickpea:}\textit{ round, beige legume often used in cooking.}

\noindent
\textbf{chili\_(vegetable):}\textit{ spicy pepper used in various cuisines.}

\noindent
\textbf{chime:}\textit{ musical instrument that produces a ringing sound.}

\noindent
\textbf{chinaware:}\textit{ decorative ceramic dishware, often used for dining.}

\noindent
\textbf{crisp\_(potato\_chip):}\textit{ thin, fried slice of potato, often crunchy.}

\noindent
\textbf{poker\_chip:}\textit{ small disc used in gambling games like poker.}

\noindent
\textbf{chocolate\_bar:}\textit{ solid confection made primarily of chocolate.}

\noindent
\textbf{chocolate\_cake:}\textit{ cake made with chocolate, often layered and frosted.}

\noindent
\textbf{chocolate\_milk:}\textit{ sweet beverage made by mixing chocolate with milk.}

\noindent
\textbf{chocolate\_mousse:}\textit{ light, creamy dessert made with chocolate.}

\noindent
\textbf{choker:}\textit{ close-fitting necklace worn around the neck.}

\noindent
\textbf{chopping\_board:}\textit{ flat surface used for cutting food.}

\noindent
\textbf{chopstick:}\textit{ pair of slender sticks used for eating asian cuisine.}

\noindent
\textbf{christmas\_tree:}\textit{ evergreen tree decorated with ornaments for the holiday.}

\noindent
\textbf{slide:}\textit{ smooth surface for sliding down, often found in playgrounds.}

\noindent
\textbf{cider:}\textit{ beverage made from pressed apples, often fermented.}

\noindent
\textbf{cigar\_box:}\textit{ container for storing cigars.}

\noindent
\textbf{cigarette:}\textit{ thin roll of tobacco for smoking.}

\noindent
\textbf{cigarette\_case:}\textit{ holder for storing cigarettes, often decorative.}

\noindent
\textbf{cistern:}\textit{ large tank for storing water.}

\noindent
\textbf{clarinet:}\textit{ woodwind instrument with a single-reed mouthpiece.}

\noindent
\textbf{clasp:}\textit{ fastening device for securing items together.}

\noindent
\textbf{cleansing\_agent:}\textit{ substance used for cleaning surfaces.}

\noindent
\textbf{cleat\_(for\_securing\_rope):}\textit{ device used to secure a rope on a boat.}

\noindent
\textbf{clementine:}\textit{ small, sweet citrus fruit, often easy to peel.}

\noindent
\textbf{clip:}\textit{ device for holding objects together, often metal or plastic.}

\noindent
\textbf{clipboard:}\textit{ board with a clip for holding papers in place.}

\noindent
\textbf{clippers\_(for\_plants):}\textit{ tool for cutting plants or flowers.}

\noindent
\textbf{cloak:}\textit{ loose outer garment worn for warmth or protection.}

\noindent
\textbf{clock:}\textit{ device for measuring and displaying time.}

\noindent
\textbf{clock\_tower:}\textit{ tall structure housing a clock, often in public spaces.}

\noindent
\textbf{clothes\_hamper:}\textit{ container for storing dirty laundry.}

\noindent
\textbf{clothespin:}\textit{ wooden or plastic clip for hanging clothes to dry.}

\noindent
\textbf{clutch\_bag:}\textit{ small handbag designed to be held in hand.}

\noindent
\textbf{coaster:}\textit{ small mat for placing drinks to protect surfaces.}

\noindent
\textbf{coat:}\textit{ outer garment worn for warmth or protection.}

\noindent
\textbf{coat\_hanger:}\textit{ device for hanging coats to prevent wrinkling.}

\noindent
\textbf{coatrack:}\textit{ furniture piece for hanging coats and jackets.}

\noindent
\textbf{cock:}\textit{ male bird, often used in reference to roosters.}

\noindent
\textbf{cockroach:}\textit{ brown, flattened insect known for its resilience.}

\noindent
\textbf{cocoa\_(beverage):}\textit{ hot drink made from cocoa powder and milk.}

\noindent
\textbf{coconut:}\textit{ hard-shelled fruit with a brown outer husk and white flesh.}

\noindent
\textbf{coffee\_maker:}\textit{ appliance for brewing coffee.}

\noindent
\textbf{coffee\_table:}\textit{ low table for holding drinks and snacks in living rooms.}

\noindent
\textbf{coffeepot:}\textit{ pot used for brewing and serving coffee.}

\noindent
\textbf{coil:}\textit{ spiral or circular formation of wire or material.}

\noindent
\textbf{coin:}\textit{ small, round piece of metal used as currency.}

\noindent
\textbf{colander:}\textit{ bowl with holes for draining liquids from food.}

\noindent
\textbf{coleslaw:}\textit{ salad made from shredded cabbage and dressing.}

\noindent
\textbf{coloring\_material:}\textit{ substances used for coloring, such as crayons or markers.}

\noindent
\textbf{combination\_lock:}\textit{ lock that requires a specific sequence of numbers to open.}

\noindent
\textbf{pacifier:}\textit{ rubber or plastic device given to infants for sucking.}

\noindent
\textbf{comic\_book:}\textit{ illustrated publication that tells a story in comic form.}

\noindent
\textbf{compass:}\textit{ tool used for navigation, indicating direction.}

\noindent
\textbf{computer\_keyboard:}\textit{ input device with keys for typing.}

\noindent
\textbf{condiment:}\textit{ substance added to food for flavor, such as ketchup.}

\noindent
\textbf{cone:}\textit{ geometric shape tapering to a point, often used for ice cream.}

\noindent
\textbf{control:}\textit{ device or mechanism used to regulate something.}

\noindent
\textbf{convertible\_(automobile):}\textit{ car with a roof that can be folded down.}

\noindent
\textbf{sofa\_bed:}\textit{ couch that can be converted into a bed.}

\noindent
\textbf{cooker:}\textit{ appliance used for cooking food.}

\noindent
\textbf{cookie:}\textit{ sweet baked treat, often round and flat.}

\noindent
\textbf{cooking\_utensil:}\textit{ tool used in the kitchen for preparing food.}

\noindent
\textbf{cooler\_(for\_food):}\textit{ insulated container for keeping food and drinks cold.}

\noindent
\textbf{cork\_(bottle\_plug):}\textit{ plug used to seal a bottle, usually made of cork.}

\noindent
\textbf{corkboard:}\textit{ board covered with cork for pinning notes and messages.}

\noindent
\textbf{corkscrew:}\textit{ tool for removing corks from bottles.}

\noindent
\textbf{edible\_corn:}\textit{ yellow grain that can be eaten, often used as food.}

\noindent
\textbf{cornbread:}\textit{ bread made from cornmeal, typically sweet and dense.}

\noindent
\textbf{cornet:}\textit{ musical instrument resembling a trumpet.}

\noindent
\textbf{cornice:}\textit{ decorative molding at the top of a wall or building.}

\noindent
\textbf{cornmeal:}\textit{ ground corn used in cooking and baking.}

\noindent
\textbf{corset:}\textit{ garment worn to shape the waist.}

\noindent
\textbf{costume:}\textit{ outfit worn for a particular occasion or role.}

\noindent
\textbf{cougar:}\textit{ large wild cat known for its agility and stealth.}

\noindent
\textbf{coverall:}\textit{ one-piece garment worn for protection, often in work environments.}

\noindent
\textbf{cowbell:}\textit{ bell hung around a cow’s neck to locate it.}

\noindent
\textbf{cowboy\_hat:}\textit{ wide-brimmed hat associated with cowboy culture.}

\noindent
\textbf{crab\_(animal):}\textit{ shellfish with a hard shell and pincers.}

\noindent
\textbf{crabmeat:}\textit{ meat from crabs, often used in cooking.}

\noindent
\textbf{cracker:}\textit{ crisp, dry biscuit often eaten with cheese or dips.}

\noindent
\textbf{crape:}\textit{ thin, textured fabric used in clothing and decorations.}

\noindent
\textbf{crate:}\textit{ wooden or plastic container for transporting goods.}

\noindent
\textbf{crayon:}\textit{ colored wax stick used for drawing and coloring.}

\noindent
\textbf{cream\_pitcher:}\textit{ small container for serving cream.}

\noindent
\textbf{crescent\_roll:}\textit{ soft, flaky pastry shaped like a crescent.}

\noindent
\textbf{crib:}\textit{ bed for a baby or small child.}

\noindent
\textbf{crock\_pot:}\textit{ slow cooker for preparing meals over time.}

\noindent
\textbf{crossbar:}\textit{ bar used for support or as a boundary.}

\noindent
\textbf{crouton:}\textit{ small, crispy bread piece often used in salads.}

\noindent
\textbf{crow:}\textit{ large, black bird known for its intelligence.}

\noindent
\textbf{crowbar:}\textit{ tool used for prying and lifting objects.}

\noindent
\textbf{crown:}\textit{ ornamental headpiece worn as a symbol of authority.}

\noindent
\textbf{crucifix:}\textit{ cross with a representation of jesus, used in christianity.}

\noindent
\textbf{cruise\_ship:}\textit{ large vessel designed for leisure travel on the water.}

\noindent
\textbf{police\_cruiser:}\textit{ vehicle used by police for patrol and response.}

\noindent
\textbf{crumb:}\textit{ small piece or fragment of baked goods.}

\noindent
\textbf{crutch:}\textit{ supportive device used to aid walking.}

\noindent
\textbf{cub\_(animal):}\textit{ young animal, especially of bears or big cats.}

\noindent
\textbf{cube:}\textit{ solid, three-dimensional shape with six equal square faces.}

\noindent
\textbf{cucumber:}\textit{ long, green vegetable, often used in salads.}

\noindent
\textbf{cufflink:}\textit{ decorative fastener used to secure the cuffs of a shirt.}

\noindent
\textbf{cup:}\textit{ small, typically cylindrical container for drinking.}

\noindent
\textbf{trophy\_cup:}\textit{ award given for achievement, usually in sports.}

\noindent
\textbf{cupboard:}\textit{ storage cabinet with shelves for dishes and food.}

\noindent
\textbf{cupcake:}\textit{ small cake baked in a cup, often frosted.}

\noindent
\textbf{hair\_curler:}\textit{ device used to curl hair into waves or spirals.}

\noindent
\textbf{curling\_iron:}\textit{ heated tool for curling hair.}

\noindent
\textbf{curtain:}\textit{ fabric panel hung to cover windows or divide rooms.}

\noindent
\textbf{cushion:}\textit{ soft pad used for comfort, often on furniture.}

\noindent
\textbf{cylinder:}\textit{ three-dimensional shape with circular bases.}

\noindent
\textbf{cymbal:}\textit{ musical instrument that produces a crashing sound.}

\noindent
\textbf{dagger:}\textit{ short, pointed knife used as a weapon.}

\noindent
\textbf{dalmatian:}\textit{ breed of dog known for its distinctive black spots.}

\noindent
\textbf{dartboard:}\textit{ board used for playing darts, marked with scores.}

\noindent
\textbf{date\_(fruit):}\textit{ sweet, chewy fruit from the date palm.}

\noindent
\textbf{deck\_chair:}\textit{ folding chair designed for outdoor use.}

\noindent
\textbf{deer:}\textit{ hoofed animal known for its graceful movements.}

\noindent
\textbf{dental\_floss:}\textit{ thin string used for cleaning between teeth.}

\noindent
\textbf{desk:}\textit{ surface for working, often with drawers for storage.}

\noindent
\textbf{detergent:}\textit{ cleaning agent used for laundry and dishes.}

\noindent
\textbf{diaper:}\textit{ absorbent garment worn by infants.}

\noindent
\textbf{diary:}\textit{ book for recording daily thoughts and events.}

\noindent
\textbf{die:}\textit{ cube used in games for generating random numbers.}

\noindent
\textbf{dinghy:}\textit{ small boat, often used for short trips or as a tender.}

\noindent
\textbf{dining\_table:}\textit{ table used for eating meals.}

\noindent
\textbf{tux:}\textit{ formal suit typically worn for black-tie events.}

\noindent
\textbf{dish:}\textit{ shallow container for serving or cooking food.}

\noindent
\textbf{dish\_antenna:}\textit{ satellite dish used for receiving signals.}

\noindent
\textbf{dishrag:}\textit{ cloth used for cleaning dishes.}

\noindent
\textbf{dishtowel:}\textit{ towel used for drying dishes and utensils.}

\noindent
\textbf{dishwasher:}\textit{ appliance for automatically washing dishes.}

\noindent
\textbf{dishwasher\_detergent:}\textit{ cleaning agent used in dishwashers.}

\noindent
\textbf{dispenser:}\textit{ device for distributing a product, like soap or food.}

\noindent
\textbf{diving\_board:}\textit{ springboard for jumping into a swimming pool.}

\noindent
\textbf{dixie\_cup:}\textit{ small paper cup often used for serving drinks.}

\noindent
\textbf{dog:}\textit{ domesticated animal known for companionship and loyalty.}

\noindent
\textbf{dog\_collar:}\textit{ strap worn around a dog’s neck, often for identification.}

\noindent
\textbf{doll:}\textit{ toy figure representing a human, often used for play.}

\noindent
\textbf{dollar:}\textit{ unit of currency used in the united states and other countries.}

\noindent
\textbf{dollhouse:}\textit{ miniature house designed for dolls and toys.}

\noindent
\textbf{dolphin:}\textit{ intelligent marine mammal known for its playful nature.}

\noindent
\textbf{domestic\_ass:}\textit{ donkey used for work and companionship.}

\noindent
\textbf{doorknob:}\textit{ handle used for opening and closing doors.}

\noindent
\textbf{doormat:}\textit{ mat placed at the entrance to a home for wiping feet.}

\noindent
\textbf{doughnut:}\textit{ fried sweet pastry, often ring-shaped.}

\noindent
\textbf{dove:}\textit{ bird symbolizing peace, often white in color.}

\noindent
\textbf{dragonfly:}\textit{ insect known for its large wings and agile flight.}

\noindent
\textbf{drawer:}\textit{ compartment in furniture used for storage.}

\noindent
\textbf{underdrawers:}\textit{ underwear or undergarments.}

\noindent
\textbf{dress:}\textit{ garment worn by women, typically flowing and elegant.}

\noindent
\textbf{dress\_hat:}\textit{ formal hat worn with elegant attire.}

\noindent
\textbf{dress\_suit:}\textit{ formal outfit worn for special occasions.}

\noindent
\textbf{dresser:}\textit{ furniture piece with drawers for storing clothes.}

\noindent
\textbf{drill:}\textit{ tool used for making holes in various materials.}

\noindent
\textbf{drone:}\textit{ unmanned aerial vehicle often used for surveillance or photography.}

\noindent
\textbf{dropper:}\textit{ tool used for dispensing small amounts of liquid.}

\noindent
\textbf{drum\_(musical\_instrument):}\textit{ percussion instrument with a circular body.}

\noindent
\textbf{drumstick:}\textit{ stick used for playing a drum.}

\noindent
\textbf{duck:}\textit{ medium-sized bird with a round body, webbed feet, and a flat beak.}

\noindent
\textbf{duckling:}\textit{ small, fluffy bird with a yellow downy coat.}

\noindent
\textbf{duct\_tape:}\textit{ wide, silver or black adhesive tape with a textured surface.}

\noindent
\textbf{duffel\_bag:}\textit{ cylindrical, soft-sided bag with handles and a zipper.}

\noindent
\textbf{dumbbell:}\textit{ short bar with round weights on each end.}

\noindent
\textbf{dumpster:}\textit{ large, rectangular metal container with hinged lids.}

\noindent
\textbf{dustpan:}\textit{ flat, scoop-shaped tray with a handle.}

\noindent
\textbf{eagle:}\textit{ large bird with a hooked beak and broad wings.}

\noindent
\textbf{earphone:}\textit{ small, round device with a cord, worn in the ear for listening.}

\noindent
\textbf{earplug:}\textit{ small, cylindrical or conical foam piece designed to fit in the ear.}

\noindent
\textbf{earring:}\textit{ small piece of jewelry worn on the earlobe, often shiny or decorative.}

\noindent
\textbf{easel:}\textit{ wooden or metal stand with angled legs, used for holding canvases.}

\noindent
\textbf{eclair:}\textit{ long, puffed pastry with a glossy, chocolate-glazed top.}

\noindent
\textbf{eel:}\textit{ long, slender, snake-like fish with smooth skin.}

\noindent
\textbf{egg:}\textit{ oval-shaped, smooth, and hard-shelled object, usually white or brown.}

\noindent
\textbf{egg\_roll:}\textit{ cylindrical roll wrapped in a golden, crispy shell.}

\noindent
\textbf{egg\_yolk:}\textit{ yellow, round center of an egg.}

\noindent
\textbf{eggbeater:}\textit{ handheld whisk with rotating blades and a handle.}

\noindent
\textbf{eggplant:}\textit{ large, glossy purple vegetable with an oblong shape.}

\noindent
\textbf{electric\_chair:}\textit{ chair with metal components and straps attached.}

\noindent
\textbf{refrigerator:}\textit{ large, boxy appliance with a door and shelves inside.}

\noindent
\textbf{elephant:}\textit{ large, gray animal with a long trunk and large ears.}

\noindent
\textbf{elk:}\textit{ large deer with long antlers and a shaggy coat.}

\noindent
\textbf{envelope:}\textit{ thin, rectangular paper sleeve with a flap for sealing.}

\noindent
\textbf{eraser:}\textit{ soft, rubber block, usually pink or white.}

\noindent
\textbf{escargot:}\textit{ small snail, often served with a spiral shell.}

\noindent
\textbf{eyepatch:}\textit{ small, dark fabric piece worn over one eye.}

\noindent
\textbf{falcon:}\textit{ sleek bird with sharp talons and a pointed beak.}

\noindent
\textbf{fan:}\textit{ round or rectangular device with spinning blades inside a protective grill.}

\noindent
\textbf{faucet:}\textit{ metal fixture with a curved spout and a handle for controlling water.}

\noindent
\textbf{fedora:}\textit{ soft hat with a creased crown and a brim.}

\noindent
\textbf{ferret:}\textit{ small, slender animal with soft fur and a pointed snout.}

\noindent
\textbf{ferris\_wheel:}\textit{ large, circular structure with passenger cars attached.}

\noindent
\textbf{ferry:}\textit{ large, flat-bottomed boat with a ramp for vehicles and passengers.}

\noindent
\textbf{fig\_(fruit):}\textit{ small, round or oval fruit with a smooth purple or green skin.}

\noindent
\textbf{fighter\_jet:}\textit{ sleek aircraft with sharp wings and a pointed nose.}

\noindent
\textbf{figurine:}\textit{ small, decorative model of a person or animal.}

\noindent
\textbf{file\_cabinet:}\textit{ tall, rectangular metal cabinet with pull-out drawers.}

\noindent
\textbf{file\_(tool):}\textit{ thin, metal tool with a rough surface for smoothing.}

\noindent
\textbf{fire\_alarm:}\textit{ small, red box with a glass panel and a lever.}

\noindent
\textbf{fire\_engine:}\textit{ large, red truck with hoses and ladders attached.}

\noindent
\textbf{fire\_extinguisher:}\textit{ red, cylindrical container with a nozzle and a handle.}

\noindent
\textbf{fire\_hose:}\textit{ long, thick, flexible tube coiled around a reel.}

\noindent
\textbf{fireplace:}\textit{ brick or stone opening in a wall with a hearth for burning wood.}

\noindent
\textbf{fireplug:}\textit{ short, round metal hydrant with caps and nozzles.}

\noindent
\textbf{first-aid\_kit:}\textit{ small box with a red cross symbol, containing medical supplies.}

\noindent
\textbf{fish:}\textit{ sleek, scaly creature with fins and gills.}

\noindent
\textbf{fish\_(food):}\textit{ cooked or raw pieces of fish, often flaky or filleted.}

\noindent
\textbf{fishbowl:}\textit{ round, transparent glass container filled with water.}

\noindent
\textbf{fishing\_rod:}\textit{ long, slender pole with a reel and fishing line attached.}

\noindent
\textbf{flag:}\textit{ rectangular piece of fabric with patterns or symbols, attached to a pole.}

\noindent
\textbf{flagpole:}\textit{ tall, straight pole with a mechanism for raising a flag.}

\noindent
\textbf{flamingo:}\textit{ tall bird with pink feathers, long legs, and a curved neck.}

\noindent
\textbf{flannel:}\textit{ soft, plaid-patterned fabric, often used in shirts.}

\noindent
\textbf{flap:}\textit{ thin, flexible piece that covers an opening or edge.}

\noindent
\textbf{flash:}\textit{ bright, quick burst of light.}

\noindent
\textbf{flashlight:}\textit{ cylindrical handheld device with a lens for projecting light.}

\noindent
\textbf{fleece:}\textit{ soft, fluffy fabric, often used for warmth.}

\noindent
\textbf{flip-flop\_(sandal):}\textit{ open-toe sandal with a y-shaped strap between the toes.}

\noindent
\textbf{flipper\_(footwear):}\textit{ large, flat, flexible fin worn on the feet for swimming.}

\noindent
\textbf{flower\_arrangement:}\textit{ assorted flowers grouped together, often in a vase.}

\noindent
\textbf{flute\_glass:}\textit{ tall, slender glass with a narrow bowl for holding champagne.}

\noindent
\textbf{foal:}\textit{ young horse with a small, delicate frame and thin legs.}

\noindent
\textbf{folding\_chair:}\textit{ collapsible chair with metal or plastic legs and a fabric seat.}

\noindent
\textbf{food\_processor:}\textit{ boxy appliance with a clear bowl and rotating blades inside.}

\noindent
\textbf{football\_(american):}\textit{ oval-shaped, brown leather ball with white laces.}

\noindent
\textbf{football\_helmet:}\textit{ rounded helmet with a faceguard and chin strap.}

\noindent
\textbf{footstool:}\textit{ small, padded stool for resting feet, often square or round.}

\noindent
\textbf{fork:}\textit{ metal utensil with prongs, used for eating.}

\noindent
\textbf{forklift:}\textit{ small, heavy-duty vehicle with prongs for lifting objects.}

\noindent
\textbf{freight\_car:}\textit{ long, boxy container attached to a train, used for carrying goods.}

\noindent
\textbf{french\_toast:}\textit{ golden-brown slices of bread with a soft texture.}

\noindent
\textbf{freshener:}\textit{ small, scented item with a shape or design, used to freshen air.}

\noindent
\textbf{frisbee:}\textit{ round, flat plastic disc with a slightly concave surface.}

\noindent
\textbf{frog:}\textit{ small amphibian with smooth skin and long, strong legs.}

\noindent
\textbf{fruit\_juice:}\textit{ clear or pulpy liquid, often colorful, extracted from fruit.}

\noindent
\textbf{frying\_pan:}\textit{ flat, round metal pan with a long handle and low sides.}

\noindent
\textbf{fudge:}\textit{ dense, smooth, chocolate confection, often cut into squares.}

\noindent
\textbf{funnel:}\textit{ cone-shaped tool with a narrow spout for directing liquids.}

\noindent
\textbf{futon:}\textit{ thin, foldable mattress, often placed on a low frame.}

\noindent
\textbf{gag:}\textit{ small, restrictive device, often a strip of cloth or ball.}

\noindent
\textbf{garbage:}\textit{ unwanted or discarded waste, often a mix of materials.}

\noindent
\textbf{garbage\_truck:}\textit{ large vehicle with a compactor and a bin-lifting mechanism.}

\noindent
\textbf{garden\_hose:}\textit{ long, flexible tube with a nozzle for spraying water.}

\noindent
\textbf{gargle:}\textit{ liquid, often bubbly, swirled in the mouth.}

\noindent
\textbf{gargoyle:}\textit{ stone or metal statue of a creature, often with wings and a grotesque face.}

\noindent
\textbf{garlic:}\textit{ bulb with papery skin and multiple cloves, usually white or purple.}

\noindent
\textbf{gasmask:}\textit{ protective mask with filters and eye covers.}

\noindent
\textbf{gazelle:}\textit{ slender, graceful antelope with long legs and curved horns.}

\noindent
\textbf{gelatin:}\textit{ clear, jiggly substance, often molded into shapes.}

\noindent
\textbf{gemstone:}\textit{ small, faceted stone, usually shiny and colorful.}

\noindent
\textbf{generator:}\textit{ boxy machine with vents, used for producing electricity.}

\noindent
\textbf{giant\_panda:}\textit{ large, black-and-white bear with a round body and fluffy fur.}

\noindent
\textbf{gift\_wrap:}\textit{ brightly colored paper used to wrap presents.}

\noindent
\textbf{ginger:}\textit{ knobby, beige root with thin skin.}

\noindent
\textbf{giraffe:}\textit{ tall animal with long neck, spotted coat, and small horns.}

\noindent
\textbf{cincture:}\textit{ thin belt or cord worn around the waist, often made of fabric.}

\noindent
\textbf{glass\_(drink\_container):}\textit{ transparent container with a round body and an open top.}

\noindent
\textbf{globe:}\textit{ round model of the earth with geographical features displayed.}

\noindent
\textbf{glove:}\textit{ fitted covering for the hand, often with separate sections for fingers.}

\noindent
\textbf{goat:}\textit{ small animal with curved horns and a beard.}

\noindent
\textbf{goggles:}\textit{ protective eyewear with round lenses and a strap.}

\noindent
\textbf{goldfish:}\textit{ small, orange fish with a round body and flowing fins.}

\noindent
\textbf{golf\_club:}\textit{ long stick with a rounded end for hitting golf balls.}

\noindent
\textbf{golfcart:}\textit{ small, open vehicle with a roof and seats.}

\noindent
\textbf{gondola\_(boat):}\textit{ long, narrow boat with a flat bottom.}

\noindent
\textbf{goose:}\textit{ large bird with a long neck and webbed feet.}

\noindent
\textbf{gorilla:}\textit{ large ape with a muscular build and dark fur.}

\noindent
\textbf{gourd:}\textit{ hard-shelled fruit with a round or oblong shape.}

\noindent
\textbf{grape:}\textit{ small, round fruit, usually green or purple.}

\noindent
\textbf{grater:}\textit{ flat or boxy tool with sharp holes for shredding food.}

\noindent
\textbf{gravestone:}\textit{ flat stone slab with engraved text.}

\noindent
\textbf{gravy\_boat:}\textit{ small, curved dish with a spout.}

\noindent
\textbf{green\_bean:}\textit{ long, thin vegetable with a smooth surface.}

\noindent
\textbf{green\_onion:}\textit{ tall, thin vegetable with white and green stalks.}

\noindent
\textbf{griddle:}\textit{ flat, heated cooking surface.}

\noindent
\textbf{grill:}\textit{ metal cooking grate with open flames beneath.}

\noindent
\textbf{grits:}\textit{ coarse, creamy grain dish.}

\noindent
\textbf{grizzly:}\textit{ large bear with thick brown fur.}

\noindent
\textbf{grocery\_bag:}\textit{ paper or plastic bag for carrying food.}

\noindent
\textbf{guitar:}\textit{ stringed musical instrument with a hollow body.}

\noindent
\textbf{gull:}\textit{ medium-sized bird with white feathers and long wings.}

\noindent
\textbf{gun:}\textit{ metal weapon with a barrel and trigger.}

\noindent
\textbf{hairbrush:}\textit{ handheld tool with bristles for brushing hair.}

\noindent
\textbf{hairnet:}\textit{ thin mesh worn over hair.}

\noindent
\textbf{hairpin:}\textit{ small metal pin used to hold hair in place.}

\noindent
\textbf{halter\_top:}\textit{ sleeveless shirt tied around the neck.}

\noindent
\textbf{ham:}\textit{ thick slice of cured pork.}

\noindent
\textbf{hamburger:}\textit{ round beef patty in a bun.}

\noindent
\textbf{hammer:}\textit{ tool with a metal head and a handle.}

\noindent
\textbf{hammock:}\textit{ hanging fabric sling for resting.}

\noindent
\textbf{hamper:}\textit{ tall basket for holding laundry.}

\noindent
\textbf{hamster:}\textit{ small, fluffy rodent with short legs.}

\noindent
\textbf{hair\_dryer:}\textit{ handheld device that blows hot air.}

\noindent
\textbf{hand\_glass:}\textit{ small mirror with a handle.}

\noindent
\textbf{hand\_towel:}\textit{ small, rectangular cloth for drying hands.}

\noindent
\textbf{handcart:}\textit{ two-wheeled cart with handles.}

\noindent
\textbf{handcuff:}\textit{ metal shackles linked by a chain.}

\noindent
\textbf{handkerchief:}\textit{ small square cloth, often carried in a pocket.}

\noindent
\textbf{handle:}\textit{ part of an object held by the hand.}

\noindent
\textbf{handsaw:}\textit{ saw with a straight blade and a handle.}

\noindent
\textbf{hardback\_book:}\textit{ book with a stiff, protective cover.}

\noindent
\textbf{harmonium:}\textit{ small, box-shaped musical instrument with keys.}

\noindent
\textbf{hat:}\textit{ headwear with a brim or visor.}

\noindent
\textbf{hatbox:}\textit{ round, rigid container for storing hats.}

\noindent
\textbf{veil:}\textit{ thin fabric covering the face or head.}

\noindent
\textbf{headband:}\textit{ stretchy band worn around the forehead.}

\noindent
\textbf{headboard:}\textit{ upright panel at the head of a bed.}

\noindent
\textbf{headlight:}\textit{ bright front light on a vehicle.}

\noindent
\textbf{headscarf:}\textit{ cloth worn over the head or hair.}

\noindent
\textbf{headset:}\textit{ headphones with a microphone attached.}

\noindent
\textbf{headstall\_(for\_horses):}\textit{ leather straps placed over a horse’s head.}

\noindent
\textbf{heart:}\textit{ symbol shaped like a curved, pointed oval.}

\noindent
\textbf{heater:}\textit{ boxy device for generating heat.}

\noindent
\textbf{helicopter:}\textit{ aircraft with rotating blades on top.}

\noindent
\textbf{helmet:}\textit{ hard, protective headgear.}

\noindent
\textbf{heron:}\textit{ tall bird with long legs and a sharp beak.}

\noindent
\textbf{highchair:}\textit{ chair with a raised seat for children.}

\noindent
\textbf{hinge:}\textit{ metal joint that allows doors to swing open.}

\noindent
\textbf{hippopotamus:}\textit{ large, bulky animal with thick gray skin.}

\noindent
\textbf{hockey\_stick:}\textit{ long, curved stick for playing hockey.}

\noindent
\textbf{hog:}\textit{ large, domesticated pig.}

\noindent
\textbf{home\_plate\_(baseball):}\textit{ five-sided, flat base in baseball.}

\noindent
\textbf{honey:}\textit{ thick, golden liquid made by bees.}

\noindent
\textbf{fume\_hood:}\textit{ enclosed workstation with a vent.}

\noindent
\textbf{hook:}\textit{ curved metal piece for hanging or catching objects.}

\noindent
\textbf{hookah:}\textit{ tall, water-filled pipe with a long tube.}

\noindent
\textbf{hornet:}\textit{ large, yellow and black stinging insect.}

\noindent
\textbf{horse:}\textit{ large, four-legged animal with a mane.}

\noindent
\textbf{hose:}\textit{ long, flexible tube for directing water.}

\noindent
\textbf{hot-air\_balloon:}\textit{ large, fabric balloon with a basket beneath.}

\noindent
\textbf{hotplate:}\textit{ small, portable electric stove.}

\noindent
\textbf{hot\_sauce:}\textit{ spicy liquid condiment in a bottle.}

\noindent
\textbf{hourglass:}\textit{ glass container with sand that flows through a narrow neck.}

\noindent
\textbf{houseboat:}\textit{ boat designed for living on water.}

\noindent
\textbf{hummingbird:}\textit{ tiny bird with a long beak and rapid wing beats.}

\noindent
\textbf{hummus:}\textit{ smooth, creamy chickpea dip.}

\noindent
\textbf{polar\_bear:}\textit{ large, white bear with thick fur.}

\noindent
\textbf{icecream:}\textit{ cold, creamy dessert in various flavors.}

\noindent
\textbf{popsicle:}\textit{ frozen fruit-flavored treat on a stick.}

\noindent
\textbf{ice\_maker:}\textit{ machine that produces ice cubes.}

\noindent
\textbf{ice\_pack:}\textit{ flexible, cold pouch for pain relief.}

\noindent
\textbf{ice\_skate:}\textit{ shoe with a metal blade attached for skating.}

\noindent
\textbf{igniter:}\textit{ small device used to ignite a flame.}

\noindent
\textbf{inhaler:}\textit{ handheld device for delivering medication to the lungs.}

\noindent
\textbf{ipod:}\textit{ small portable music player.}

\noindent
\textbf{iron\_(for\_clothing):}\textit{ flat, heated tool for smoothing clothes.}

\noindent
\textbf{ironing\_board:}\textit{ long, narrow board with padding for ironing clothes.}

\noindent
\textbf{jacket:}\textit{ short, outer garment with sleeves and a zipper.}

\noindent
\textbf{jam:}\textit{ thick, sweet spread made from fruit.}

\noindent
\textbf{jar:}\textit{ cylindrical glass container with a lid.}

\noindent
\textbf{jean:}\textit{ denim pants with pockets and rivets.}

\noindent
\textbf{jeep:}\textit{ boxy, rugged vehicle with large tires.}

\noindent
\textbf{jelly\_bean:}\textit{ small, bean-shaped candy with a glossy shell.}

\noindent
\textbf{jersey:}\textit{ lightweight shirt worn for sports.}

\noindent
\textbf{jet\_plane:}\textit{ fast aircraft with a sleek body and jet engines.}

\noindent
\textbf{jewel:}\textit{ small, shiny gemstone set in jewelry.}

\noindent
\textbf{jewelry:}\textit{ decorative items like rings and necklaces, often made of metal.}

\noindent
\textbf{joystick:}\textit{ handheld control stick for video games or machines.}

\noindent
\textbf{jumpsuit:}\textit{ one-piece garment with sleeves and pants.}

\noindent
\textbf{kayak:}\textit{ narrow, lightweight boat with pointed ends.}

\noindent
\textbf{keg:}\textit{ large metal barrel with a rounded shape.}

\noindent
\textbf{kennel:}\textit{ small, enclosed shelter for dogs.}

\noindent
\textbf{kettle:}\textit{ round metal container with a spout and handle.}

\noindent
\textbf{key:}\textit{ small, flat metal piece with a jagged edge.}

\noindent
\textbf{keycard:}\textit{ flat plastic card with electronic data.}

\noindent
\textbf{kilt:}\textit{ knee-length skirt with pleats, often plaid.}

\noindent
\textbf{kimono:}\textit{ loose-fitting robe with wide sleeves.}

\noindent
\textbf{kitchen\_sink:}\textit{ shallow basin with a faucet for washing.}

\noindent
\textbf{kitchen\_table:}\textit{ flat surface with legs, used for dining.}

\noindent
\textbf{kite:}\textit{ lightweight frame with fabric stretched over it, flown in the wind.}

\noindent
\textbf{kitten:}\textit{ small, fluffy baby cat.}

\noindent
\textbf{kiwi\_fruit:}\textit{ brown, fuzzy fruit with green flesh inside.}

\noindent
\textbf{knee\_pad:}\textit{ cushioned pad for protecting the knee.}

\noindent
\textbf{knife:}\textit{ sharp metal blade with a handle.}

\noindent
\textbf{knitting\_needle:}\textit{ long, pointed stick used for knitting.}

\noindent
\textbf{knob:}\textit{ round handle or switch for turning.}

\noindent
\textbf{knocker\_(on\_a\_door):}\textit{ metal ring or bar for knocking on doors.}

\noindent
\textbf{koala:}\textit{ small, gray furry animal with large ears and a round nose.}

\noindent
\textbf{lab\_coat:}\textit{ long white coat worn by scientists.}

\noindent
\textbf{ladder:}\textit{ vertical structure with steps for climbing.}

\noindent
\textbf{ladle:}\textit{ long-handled spoon with a deep bowl.}

\noindent
\textbf{ladybug:}\textit{ small red insect with black spots.}

\noindent
\textbf{lamb\_(animal):}\textit{ young sheep with soft wool.}

\noindent
\textbf{lamb-chop:}\textit{ slice of lamb meat with a bone.}

\noindent
\textbf{lamp:}\textit{ light source with a bulb and a shade.}

\noindent
\textbf{lamppost:}\textit{ tall post with a light on top.}

\noindent
\textbf{lampshade:}\textit{ cover for a light bulb, usually conical or cylindrical.}

\noindent
\textbf{lantern:}\textit{ portable light with a handle and enclosed flame or bulb.}

\noindent
\textbf{lanyard:}\textit{ cord worn around the neck for holding items.}

\noindent
\textbf{laptop\_computer:}\textit{ portable computer with a foldable screen and keyboard.}

\noindent
\textbf{lasagna:}\textit{ layered pasta dish with sauce and cheese.}

\noindent
\textbf{latch:}\textit{ metal fastener for securing doors or gates.}

\noindent
\textbf{lawn\_mower:}\textit{ machine with rotating blades for cutting grass.}

\noindent
\textbf{leather:}\textit{ smooth, flexible material made from animal hide.}

\noindent
\textbf{legging\_(clothing):}\textit{ tight-fitting pants, often stretchy.}

\noindent
\textbf{lego:}\textit{ small, colorful plastic building blocks.}

\noindent
\textbf{legume:}\textit{ edible seed or pod, like beans or peas.}

\noindent
\textbf{lemon:}\textit{ small, yellow citrus fruit with a bumpy skin.}

\noindent
\textbf{lemonade:}\textit{ sweet, yellow drink made from lemons.}

\noindent
\textbf{lettuce:}\textit{ leafy green vegetable with a crisp texture.}

\noindent
\textbf{license\_plate:}\textit{ metal plate with letters and numbers on vehicles.}

\noindent
\textbf{life\_buoy:}\textit{ ring-shaped flotation device used for rescue.}

\noindent
\textbf{life\_jacket:}\textit{ padded vest worn for flotation in water.}

\noindent
\textbf{lightbulb:}\textit{ glass bulb that produces light when powered.}

\noindent
\textbf{lightning\_rod:}\textit{ metal rod placed on buildings to prevent lightning damage.}

\noindent
\textbf{lime:}\textit{ small, green citrus fruit with a sour taste.}

\noindent
\textbf{limousine:}\textit{ long, luxurious car with multiple doors.}

\noindent
\textbf{lion:}\textit{ large, muscular animal with a mane and a tawny coat.}

\noindent
\textbf{lip\_balm:}\textit{ small stick or tube of moisturizing substance for lips.}

\noindent
\textbf{liquor:}\textit{ clear or amber-colored alcoholic beverage in a bottle.}

\noindent
\textbf{lizard:}\textit{ small reptile with scaly skin and a long tail.}

\noindent
\textbf{log:}\textit{ thick, solid piece of wood from a tree trunk.}

\noindent
\textbf{lollipop:}\textit{ hard candy on a stick.}

\noindent
\textbf{speaker\_(stereo\_equipment):}\textit{ boxy device that emits sound.}

\noindent
\textbf{loveseat:}\textit{ small, cushioned sofa for two people.}

\noindent
\textbf{machine\_gun:}\textit{ long-barreled gun with rapid-fire capability.}

\noindent
\textbf{magazine:}\textit{ thin booklet filled with articles and images.}

\noindent
\textbf{magnet:}\textit{ small, metallic object that attracts or repels metal.}

\noindent
\textbf{mail\_slot:}\textit{ narrow opening in a door for delivering mail.}

\noindent
\textbf{mailbox\_(at\_home):}\textit{ metal or plastic box for receiving mail.}

\noindent
\textbf{mallard:}\textit{ duck with a green head and a brown body.}

\noindent
\textbf{mallet:}\textit{ hammer with a large, soft head.}

\noindent
\textbf{mammoth:}\textit{ large, woolly prehistoric elephant-like animal.}

\noindent
\textbf{manatee:}\textit{ large, gray aquatic mammal with flippers.}

\noindent
\textbf{mandarin\_orange:}\textit{ small, round orange citrus fruit with loose skin.}

\noindent
\textbf{manger:}\textit{ trough for feeding animals, typically found in stables.}

\noindent
\textbf{manhole:}\textit{ round opening in the ground with a metal cover.}

\noindent
\textbf{map:}\textit{ flat representation of geographic areas.}

\noindent
\textbf{marker:}\textit{ thick pen with colorful ink.}

\noindent
\textbf{martini:}\textit{ clear alcoholic drink served in a wide glass.}

\noindent
\textbf{mascot:}\textit{ character or symbol representing a team or organization.}

\noindent
\textbf{mashed\_potato:}\textit{ soft, smooth dish made from cooked potatoes.}

\noindent
\textbf{masher:}\textit{ utensil with a flat, grid-like head for mashing food.}

\noindent
\textbf{mask:}\textit{ covering for the face, often with eye holes.}

\noindent
\textbf{mast:}\textit{ tall vertical pole on a ship, supporting sails.}

\noindent
\textbf{mat\_(gym\_equipment):}\textit{ flat, cushioned surface for exercise.}

\noindent
\textbf{matchbox:}\textit{ small, rectangular box for holding matches.}

\noindent
\textbf{mattress:}\textit{ thick, padded cushion for sleeping.}

\noindent
\textbf{measuring\_cup:}\textit{ cup with markings for measuring ingredients.}

\noindent
\textbf{measuring\_stick:}\textit{ long stick with markings for measuring length.}

\noindent
\textbf{meatball:}\textit{ round ball of ground meat, usually cooked.}

\noindent
\textbf{medicine:}\textit{ small, solid pills or liquid in a bottle for treatment.}

\noindent
\textbf{melon:}\textit{ large, round fruit with a hard rind and sweet flesh.}

\noindent
\textbf{microphone:}\textit{ small, handheld device for amplifying sound.}

\noindent
\textbf{microscope:}\textit{ optical device with lenses for viewing tiny objects.}

\noindent
\textbf{microwave\_oven:}\textit{ box-shaped appliance for quickly heating food.}

\noindent
\textbf{milestone:}\textit{ small, cylindrical stone marker for measuring distance.}

\noindent
\textbf{milk:}\textit{ white, liquid dairy product in a container.}

\noindent
\textbf{milk\_can:}\textit{ tall, round metal container for holding milk.}

\noindent
\textbf{milkshake:}\textit{ cold, creamy drink made from milk and ice cream.}

\noindent
\textbf{minivan:}\textit{ boxy, spacious vehicle with sliding doors.}

\noindent
\textbf{mint\_candy:}\textit{ small, round candy with a minty flavor.}

\noindent
\textbf{mirror:}\textit{ flat, reflective surface, usually framed.}

\noindent
\textbf{mitten:}\textit{ handwear with a single compartment for the fingers.}

\noindent
\textbf{mixer\_(kitchen\_tool):}\textit{ handheld or stand appliance with rotating beaters.}

\noindent
\textbf{money:}\textit{ paper bills or metal coins used for transactions.}

\noindent
\textbf{monitor\_(computer\_equipment) computer\_monitor:}\textit{ flat screen for displaying computer output.}

\noindent
\textbf{monkey:}\textit{ small, agile primate with a long tail.}

\noindent
\textbf{motor:}\textit{ box-shaped device that produces mechanical power.}

\noindent
\textbf{motor\_scooter:}\textit{ compact, two-wheeled vehicle with a small frame and wide seat.}

\noindent
\textbf{motor\_vehicle:}\textit{ large, enclosed vehicle with wheels, typically rectangular or streamlined.}

\noindent
\textbf{motorcycle:}\textit{ two-wheeled, streamlined vehicle with exposed engine and handlebars.}

\noindent
\textbf{mound\_(baseball):}\textit{ slightly elevated, round, grassy surface.}

\noindent
\textbf{mouse\_(computer\_equipment):}\textit{ small, curved device with a smooth surface and buttons.}

\noindent
\textbf{mousepad:}\textit{ thin, flat rectangular surface, often with a soft texture.}

\noindent
\textbf{muffin:}\textit{ small, round, domed baked good with a crinkled surface.}

\noindent
\textbf{mug:}\textit{ cylindrical container with a handle and thick sides.}

\noindent
\textbf{mushroom:}\textit{ rounded cap on a thin, cylindrical stem.}

\noindent
\textbf{music\_stool:}\textit{ simple, round or square seat with three or four legs.}

\noindent
\textbf{musical\_instrument:}\textit{ various shapes; generally wooden or metal with buttons, strings, or keys.}

\noindent
\textbf{nailfile:}\textit{ long, thin, flat tool with a rough surface.}

\noindent
\textbf{napkin:}\textit{ soft, square piece of cloth or paper, often folded.}

\noindent
\textbf{neckerchief:}\textit{ triangular or square cloth tied around the neck.}

\noindent
\textbf{necklace:}\textit{ thin, looped chain or string with small decorative items.}

\noindent
\textbf{necktie:}\textit{ long, narrow fabric strip, often pointed at one end.}

\noindent
\textbf{needle:}\textit{ thin, pointed metal rod.}

\noindent
\textbf{nest:}\textit{ woven or layered structure, often circular.}

\noindent
\textbf{newspaper:}\textit{ thin, rectangular, folded sheets of printed paper.}

\noindent
\textbf{newsstand:}\textit{ tall, square or rectangular display rack with shelves.}

\noindent
\textbf{nightshirt:}\textit{ loose-fitting, long-sleeved shirt.}

\noindent
\textbf{nosebag\_(for\_animals):}\textit{ round, soft fabric container with straps.}

\noindent
\textbf{noseband\_(for\_animals):}\textit{ thin strap placed around the muzzle.}

\noindent
\textbf{notebook:}\textit{ flat, rectangular object with pages bound together.}

\noindent
\textbf{notepad:}\textit{ small, square or rectangular pad with blank pages.}

\noindent
\textbf{nut:}\textit{ small, hard-shelled object, typically round.}

\noindent
\textbf{nutcracker:}\textit{ metal or wooden device with a handle and hinged mechanism.}

\noindent
\textbf{oar:}\textit{ long, wooden pole with a wide, flat end.}

\noindent
\textbf{octopus\_(food):}\textit{ curled tentacles with suction cups and a glossy surface.}

\noindent
\textbf{octopus\_(animal):}\textit{ round body with long, smooth tentacles.}

\noindent
\textbf{oil\_lamp:}\textit{ glass or metal container with a wick and curved body.}

\noindent
\textbf{olive\_oil:}\textit{ smooth, greenish-yellow liquid in a clear bottle.}

\noindent
\textbf{omelet:}\textit{ flat, folded, fluffy dish with a golden surface.}

\noindent
\textbf{onion:}\textit{ round, layered vegetable with a papery skin.}

\noindent
\textbf{orange\_(fruit):}\textit{ round, bright orange fruit with a textured skin.}

\noindent
\textbf{orange\_juice:}\textit{ yellowish liquid, often in a clear glass.}

\noindent
\textbf{ostrich:}\textit{ tall bird with long neck, fluffy body, and strong legs.}

\noindent
\textbf{ottoman:}\textit{ soft, rectangular or square padded footrest.}

\noindent
\textbf{oven:}\textit{ large, rectangular metal appliance with a front door and knobs.}

\noindent
\textbf{overalls\_(clothing):}\textit{ one-piece garment with straps and multiple pockets.}

\noindent
\textbf{owl:}\textit{ small, round bird with large eyes and feathery tufts.}

\noindent
\textbf{packet:}\textit{ small, flat, rectangular or square pouch.}

\noindent
\textbf{inkpad:}\textit{ small, flat container with a spongy ink surface.}

\noindent
\textbf{pad:}\textit{ soft, square or rectangular cushion.}

\noindent
\textbf{paddle:}\textit{ long, flat wooden or plastic tool with a wide, flat end.}

\noindent
\textbf{padlock:}\textit{ small, metallic, rectangular lock with a u-shaped shackle.}

\noindent
\textbf{paintbrush:}\textit{ thin, cylindrical handle with soft bristles at one end.}

\noindent
\textbf{painting:}\textit{ flat, rectangular surface with colorful images or designs.}

\noindent
\textbf{pajamas:}\textit{ loose-fitting, soft two-piece clothing set.}

\noindent
\textbf{palette:}\textit{ flat, oval surface with paint dabs.}

\noindent
\textbf{pan\_(for\_cooking):}\textit{ round, shallow metal container with a handle.}

\noindent
\textbf{pan\_(metal\_container):}\textit{ square or rectangular metal box for holding or cooking items.}

\noindent
\textbf{pancake:}\textit{ flat, round, golden-brown cooked batter.}

\noindent
\textbf{pantyhose:}\textit{ thin, stretchy fabric in long, leg-shaped tubes.}

\noindent
\textbf{papaya:}\textit{ oval fruit with greenish-yellow skin and orange flesh inside.}

\noindent
\textbf{paper\_plate:}\textit{ flat, round, lightweight disposable plate.}

\noindent
\textbf{paper\_towel:}\textit{ long, rectangular piece of absorbent paper.}

\noindent
\textbf{paperback\_book:}\textit{ thin, rectangular book with a flexible cover.}

\noindent
\textbf{paperweight:}\textit{ small, heavy, decorative object used to hold papers.}

\noindent
\textbf{parachute:}\textit{ large, round fabric canopy with thin ropes attached.}

\noindent
\textbf{parakeet:}\textit{ small, colorful bird with long tail feathers.}

\noindent
\textbf{parasail\_(sports):}\textit{ large, colorful parachute with ropes attached to a harness.}

\noindent
\textbf{parasol:}\textit{ small, round umbrella with a thin handle.}

\noindent
\textbf{parchment:}\textit{ thin, flat, beige or white paper-like sheet.}

\noindent
\textbf{parka:}\textit{ long, insulated jacket with a hood.}

\noindent
\textbf{parking\_meter:}\textit{ tall, thin post with a round, metal head.}

\noindent
\textbf{parrot:}\textit{ brightly colored bird with a curved beak.}

\noindent
\textbf{passenger\_car\_(part\_of\_a\_train):}\textit{ long, rectangular vehicle with rows of windows.}

\noindent
\textbf{passenger\_ship:}\textit{ large, multi-decked boat with windows and cabins.}

\noindent
\textbf{passport:}\textit{ small, rectangular booklet with a hard cover.}

\noindent
\textbf{pastry:}\textit{ small, flaky, golden-brown baked item.}

\noindent
\textbf{patty\_(food):}\textit{ round, flat, cooked food item.}

\noindent
\textbf{pea\_(food):}\textit{ small, round, green vegetable.}

\noindent
\textbf{peach:}\textit{ round, fuzzy fruit with a reddish-yellow color.}

\noindent
\textbf{peanut\_butter:}\textit{ thick, smooth or chunky brown paste.}

\noindent
\textbf{pear:}\textit{ teardrop-shaped, smooth-skinned fruit.}

\noindent
\textbf{peeler\_(tool\_for\_fruit\_and\_vegetables):}\textit{ small tool with a handle and a curved blade.}

\noindent
\textbf{wooden\_leg:}\textit{ long, cylindrical piece of wood shaped like a leg.}

\noindent
\textbf{pegboard:}\textit{ large, flat board with regularly spaced holes.}

\noindent
\textbf{pelican:}\textit{ large bird with a long bill and a pouch under the beak.}

\noindent
\textbf{pen:}\textit{ thin, cylindrical writing instrument with a pointed tip.}

\noindent
\textbf{pencil:}\textit{ slim, cylindrical stick with a graphite core and wooden body.}

\noindent
\textbf{pencil\_box:}\textit{ small, rectangular container for holding pencils.}

\noindent
\textbf{pencil\_sharpener:}\textit{ small, rectangular or cylindrical device with a blade for sharpening pencils.}

\noindent
\textbf{pendulum:}\textit{ long, thin rod or string with a weight at the end.}

\noindent
\textbf{penguin:}\textit{ short, stocky bird with black and white feathers.}

\noindent
\textbf{pennant:}\textit{ triangular fabric flag attached to a stick or string.}

\noindent
\textbf{penny\_(coin):}\textit{ small, round, copper-colored coin.}

\noindent
\textbf{pepper:}\textit{ small, round or long vegetable, smooth or wrinkled skin.}

\noindent
\textbf{pepper\_mill:}\textit{ tall, cylindrical container with a rotating top for grinding pepper.}

\noindent
\textbf{perfume:}\textit{ small, decorative glass bottle with a sprayer.}

\noindent
\textbf{persimmon:}\textit{ round, smooth-skinned orange fruit.}

\noindent
\textbf{person:}\textit{ human figure with limbs and distinct features.}

\noindent
\textbf{pet:}\textit{ small, domesticated animal with varied shapes and sizes.}

\noindent
\textbf{pew\_(church\_bench):}\textit{ long, narrow wooden bench with a high back.}

\noindent
\textbf{phonebook:}\textit{ thick, rectangular book with printed names and numbers.}

\noindent
\textbf{phonograph\_record:}\textit{ flat, round disc with grooves.}

\noindent
\textbf{piano:}\textit{ large, rectangular instrument with black and white keys.}

\noindent
\textbf{pickle:}\textit{ long, green, bumpy vegetable preserved in liquid.}

\noindent
\textbf{pickup\_truck:}\textit{ large, boxy vehicle with an open cargo bed.}

\noindent
\textbf{pie:}\textit{ round, flat pastry with a golden crust, often with a textured or lattice top.}

\noindent
\textbf{pigeon:}\textit{ small bird with a round body, smooth feathers, and a short beak.}

\noindent
\textbf{piggy\_bank:}\textit{ small, hollow, ceramic or plastic figure, often shaped like a pig, with a coin slot on top.}

\noindent
\textbf{pillow:}\textit{ soft, rectangular or square cushion with a smooth fabric covering.}

\noindent
\textbf{pin\_(non\_jewelry):}\textit{ small, thin, straight metal object with a round head.}

\noindent
\textbf{pineapple:}\textit{ large, oval-shaped fruit with rough, spiky skin and a tuft of spiky green leaves.}

\noindent
\textbf{pinecone:}\textit{ brown, scaly, conical structure with a rough texture.}

\noindent
\textbf{ping-pong\_ball:}\textit{ small, round, lightweight white or orange ball.}

\noindent
\textbf{pinwheel:}\textit{ colorful, flat, spinning paper or plastic shape on a thin stick.}

\noindent
\textbf{tobacco\_pipe:}\textit{ small, curved object with a bowl and a long stem.}

\noindent
\textbf{pipe:}\textit{ long, cylindrical tube, typically metal or plastic.}

\noindent
\textbf{pistol:}\textit{ compact, angular, metal firearm with a grip and barrel.}

\noindent
\textbf{pita\_(bread):}\textit{ round, flat bread with a slightly puffed texture.}

\noindent
\textbf{pitcher\_(vessel\_for\_liquid):}\textit{ tall, cylindrical container with a handle and spout.}

\noindent
\textbf{pitchfork:}\textit{ long handle with a metal head featuring several sharp, straight prongs.}

\noindent
\textbf{pizza:}\textit{ flat, round base topped with various colorful ingredients and a golden crust.}

\noindent
\textbf{place\_mat:}\textit{ flat, rectangular or circular mat, usually made of fabric or plastic.}

\noindent
\textbf{plate:}\textit{ flat, round dish with a slightly raised edge.}

\noindent
\textbf{platter:}\textit{ large, flat, oval or rectangular dish with raised edges.}

\noindent
\textbf{playpen:}\textit{ square or rectangular, soft-sided enclosure with mesh or plastic walls.}

\noindent
\textbf{pliers:}\textit{ handheld tool with two metal, pivoting arms ending in gripping jaws.}

\noindent
\textbf{plow\_(farm\_equipment):}\textit{ large metal blade or series of blades attached to a long frame.}

\noindent
\textbf{plume:}\textit{ long, colorful feather with a soft, fluffy texture.}

\noindent
\textbf{pocket\_watch:}\textit{ small, round, metal watch with a hinged cover and chain.}

\noindent
\textbf{pocketknife:}\textit{ small, foldable knife with a smooth, rectangular handle.}

\noindent
\textbf{poker\_(fire\_stirring\_tool):}\textit{ long, thin metal rod with a pointed tip and handle.}

\noindent
\textbf{pole:}\textit{ tall, thin, cylindrical object, often made of wood or metal.}

\noindent
\textbf{polo\_shirt:}\textit{ short-sleeved shirt with a collar and buttons near the neck.}

\noindent
\textbf{poncho:}\textit{ large, rectangular or circular piece of fabric with an opening for the head.}

\noindent
\textbf{pony:}\textit{ small, sturdy horse with a stocky build and a short mane.}

\noindent
\textbf{pool\_table:}\textit{ large, rectangular, green felt-covered table with pockets at the corners.}

\noindent
\textbf{pop\_(soda):}\textit{ clear or colored liquid in a tall, cylindrical can or bottle.}

\noindent
\textbf{postbox\_(public):}\textit{ tall, rectangular or cylindrical box with a small mail slot and a rounded top.}

\noindent
\textbf{postcard:}\textit{ small, rectangular card with a printed image on one side and space for writing on the other.}

\noindent
\textbf{poster:}\textit{ large, flat sheet of paper with images or text, often rectangular.}

\noindent
\textbf{pot:}\textit{ round, deep container with a flat base and straight or sloped sides.}

\noindent
\textbf{flowerpot:}\textit{ small, round, usually terracotta or plastic container with a flared top.}

\noindent
\textbf{potato:}\textit{ oval, rough-textured tuber with a brown or yellowish skin.}

\noindent
\textbf{potholder:}\textit{ small, flat, square piece of padded fabric with a quilted texture.}

\noindent
\textbf{pottery:}\textit{ rounded, smooth or textured objects, typically made of clay, with various shapes.}

\noindent
\textbf{pouch:}\textit{ small, soft, flat container with a drawstring or zipper.}

\noindent
\textbf{power\_shovel:}\textit{ large, heavy machine with a long arm and a large bucket at the end.}

\noindent
\textbf{prawn:}\textit{ small, elongated sea creature with a curved, segmented body and thin legs.}

\noindent
\textbf{pretzel:}\textit{ twisted, baked bread snack with a golden-brown, shiny surface.}

\noindent
\textbf{printer:}\textit{ rectangular device with buttons and paper slots, often with a flat top.}

\noindent
\textbf{projectile\_(weapon):}\textit{ small, sleek object with a pointed tip and a cylindrical or round body.}

\noindent
\textbf{projector:}\textit{ boxy device with a lens in the front, typically mounted on a stand.}

\noindent
\textbf{propeller:}\textit{ round, central hub with multiple flat blades extending outward.}

\noindent
\textbf{prune:}\textit{ small, wrinkled, dark-colored dried fruit.}

\noindent
\textbf{pudding:}\textit{ smooth, thick, creamy dessert often served in small bowls.}

\noindent
\textbf{puffer\_(fish):}\textit{ round, spiny fish with a bloated appearance when inflated.}

\noindent
\textbf{puffin:}\textit{ small bird with a black and white body and a brightly colored beak.}

\noindent
\textbf{pug-dog:}\textit{ small dog with a wrinkled face, short snout, and curled tail.}

\noindent
\textbf{pumpkin:}\textit{ large, round, orange fruit with a smooth, ridged surface.}

\noindent
\textbf{puncher:}\textit{ small, metal device with a handle and circular punching mechanism.}

\noindent
\textbf{puppet:}\textit{ small, soft figure with strings or hand controls for movement.}

\noindent
\textbf{puppy:}\textit{ small, fluffy young dog with large eyes and short legs.}

\noindent
\textbf{quesadilla:}\textit{ flat, round tortilla filled with melted cheese and other ingredients.}

\noindent
\textbf{quiche:}\textit{ round, golden-brown pastry filled with egg and other ingredients.}

\noindent
\textbf{quilt:}\textit{ large, rectangular blanket made of small, colorful fabric patches.}

\noindent
\textbf{rabbit:}\textit{ small, furry animal with long ears and a short, fluffy tail.}

\noindent
\textbf{race\_car:}\textit{ low, sleek vehicle with a streamlined body and large tires.}

\noindent
\textbf{racket:}\textit{ oval frame with a tight web of strings attached to a long handle.}

\noindent
\textbf{radar:}\textit{ large, flat or round dish mounted on a stand or structure.}

\noindent
\textbf{radiator:}\textit{ rectangular metal panel with a series of vertical or horizontal fins.}

\noindent
\textbf{radio\_receiver:}\textit{ rectangular or square device with dials and a small antenna.}

\noindent
\textbf{radish:}\textit{ small, round or oval root vegetable with a smooth red or white skin.}

\noindent
\textbf{raft:}\textit{ flat, rectangular inflatable or wooden platform for floating.}

\noindent
\textbf{rag\_doll:}\textit{ soft, fabric doll with stitched features and loose limbs.}

\noindent
\textbf{raincoat:}\textit{ long, waterproof jacket with a smooth, shiny surface.}

\noindent
\textbf{ram\_(animal):}\textit{ sturdy, woolly animal with large, curved horns.}

\noindent
\textbf{raspberry:}\textit{ small, round, red fruit made up of tiny clusters.}

\noindent
\textbf{rat:}\textit{ small rodent with a long tail, pointed nose, and short fur.}

\noindent
\textbf{razorblade:}\textit{ thin, flat piece of metal with a sharp edge.}

\noindent
\textbf{reamer\_(juicer):}\textit{ small, pointed, ridged tool for extracting juice.}

\noindent
\textbf{rearview\_mirror:}\textit{ small, rectangular mirror mounted inside a vehicle.}

\noindent
\textbf{receipt:}\textit{ long, narrow piece of paper with printed text.}

\noindent
\textbf{recliner:}\textit{ large, padded chair with a footrest and adjustable back.}

\noindent
\textbf{record\_player:}\textit{ large, flat device with a spinning turntable and a needle arm.}

\noindent
\textbf{reflector:}\textit{ small, round or rectangular object with a shiny or reflective surface.}

\noindent
\textbf{remote\_control:}\textit{ small, rectangular device with buttons and a smooth surface.}

\noindent
\textbf{rhinoceros:}\textit{ large, thick-skinned animal with one or two horns on its snout.}

\noindent
\textbf{rib\_(food):}\textit{ curved bone with a layer of cooked meat attached.}

\noindent
\textbf{rifle:}\textit{ long, slender firearm with a smooth barrel and stock.}

\noindent
\textbf{ring:}\textit{ small, circular band of metal or other material.}

\noindent
\textbf{river\_boat:}\textit{ long, flat vessel with a shallow draft and a wide deck.}

\noindent
\textbf{road\_map:}\textit{ large, flat, folded paper with printed lines and symbols.}

\noindent
\textbf{robe:}\textit{ long, loose-fitting garment with a belt and wide sleeves.}

\noindent
\textbf{rocking\_chair:}\textit{ wooden or padded chair with curved, arched rockers at the base.}

\noindent
\textbf{rodent:}\textit{ small, furry animal with a pointed nose and long tail.}

\noindent
\textbf{roller\_skate:}\textit{ shoe with four wheels attached to the bottom in two rows.}

\noindent
\textbf{rollerblade:}\textit{ boot with a single row of wheels attached to the sole.}

\noindent
\textbf{rolling\_pin:}\textit{ long, cylindrical tool with handles on each end.}

\noindent
\textbf{root\_beer:}\textit{ dark, foamy beverage in a glass or bottle.}

\noindent
\textbf{router\_(computer\_equipment):}\textit{ small, boxy device with antennas and lights on the front.}

\noindent
\textbf{rubber\_band:}\textit{ thin, flat, stretchy loop of rubber.}

\noindent
\textbf{runner\_(carpet):}\textit{ long, narrow strip of carpet with bound edges.}

\noindent
\textbf{plastic\_bag:}\textit{ thin, transparent or colored, flexible bag with handles.}

\noindent
\textbf{saddle\_(on\_an\_animal):}\textit{ curved leather seat with stirrups attached.}

\noindent
\textbf{saddle\_blanket:}\textit{ rectangular, thick fabric pad placed under a saddle.}

\noindent
\textbf{saddlebag:}\textit{ soft, rectangular bag that hangs from a saddle, often with buckles.}

\noindent
\textbf{safety\_pin:}\textit{ small, thin metal pin with a coil and a clasp at one end.}

\noindent
\textbf{sail:}\textit{ large, flat, triangular or rectangular fabric stretched between poles.}

\noindent
\textbf{salad:}\textit{ colorful mixture of vegetables, usually with green leaves.}

\noindent
\textbf{salad\_plate:}\textit{ small, round plate, often with a slight rim.}

\noindent
\textbf{salami:}\textit{ cylindrical sausage with a textured, dark red exterior.}

\noindent
\textbf{salmon\_(fish):}\textit{ streamlined fish with a silvery body and pinkish scales.}

\noindent
\textbf{salmon\_(food):}\textit{ pink, flaky fish meat often served in slices or fillets.}

\noindent
\textbf{salsa:}\textit{ bright, chunky mixture of chopped vegetables or fruit in a bowl.}

\noindent
\textbf{saltshaker:}\textit{ small, round container with holes on top for dispensing salt.}

\noindent
\textbf{sandal\_(type\_of\_shoe):}\textit{ open shoe with straps across the foot and around the heel.}

\noindent
\textbf{sandwich:}\textit{ two pieces of bread with various fillings inside.}

\noindent
\textbf{satchel:}\textit{ soft, rectangular bag with a long strap, usually worn over the shoulder.}

\noindent
\textbf{saucepan:}\textit{ deep, round metal pan with a long handle.}

\noindent
\textbf{saucer:}\textit{ small, round plate with a slight indentation for a cup.}

\noindent
\textbf{sausage:}\textit{ cylindrical meat with a smooth, shiny skin.}

\noindent
\textbf{sawhorse:}\textit{ a-frame stand with a flat top used to support wood.}

\noindent
\textbf{saxophone:}\textit{ shiny, curved metal instrument with a series of buttons and a mouthpiece.}

\noindent
\textbf{scale\_(measuring\_instrument):}\textit{ flat platform with a display screen and buttons.}

\noindent
\textbf{scarecrow:}\textit{ human-like figure with clothes and straw limbs, often mounted on a stick.}

\noindent
\textbf{scarf:}\textit{ long, soft piece of fabric worn around the neck.}

\noindent
\textbf{school\_bus:}\textit{ long, rectangular vehicle, typically yellow, with rows of windows.}

\noindent
\textbf{scissors:}\textit{ two metal blades connected by a pivot, with handles for cutting.}

\noindent
\textbf{scoreboard:}\textit{ large, flat panel with numbers or lights for displaying scores.}

\noindent
\textbf{scraper:}\textit{ flat, thin tool with a sharp edge for scraping surfaces.}

\noindent
\textbf{screwdriver:}\textit{ tool with a long, narrow shaft and a handle, often with a flat or cross tip.}

\noindent
\textbf{scrubbing\_brush:}\textit{ small brush with stiff bristles and a short handle.}

\noindent
\textbf{sculpture:}\textit{ solid, three-dimensional artwork made from stone, metal, or other materials.}

\noindent
\textbf{seabird:}\textit{ medium-sized bird with sleek feathers and long wings.}

\noindent
\textbf{seahorse:}\textit{ small, curved-bodied sea creature with a long tail and a horse-like head.}

\noindent
\textbf{seaplane:}\textit{ small airplane with floats or pontoons for landing on water.}

\noindent
\textbf{seashell:}\textit{ small, smooth or ridged shell with a spiral or fan shape.}

\noindent
\textbf{sewing\_machine:}\textit{ boxy device with a needle, thread spool, and a flat working surface.}

\noindent
\textbf{shaker:}\textit{ small, round container used to shake and sprinkle spices or condiments.}

\noindent
\textbf{shampoo:}\textit{ tall, cylindrical bottle with a flip cap, containing liquid soap.}

\noindent
\textbf{shark:}\textit{ large, sleek fish with a pointed fin and sharp teeth.}

\noindent
\textbf{sharpener:}\textit{ small device with a hole for inserting pencils, often with a sharp blade inside.}

\noindent
\textbf{sharpie:}\textit{ thin, cylindrical marker with a pointed tip.}

\noindent
\textbf{shaver\_(electric):}\textit{ handheld device with rotating or oscillating blades for trimming hair.}

\noindent
\textbf{shaving\_cream:}\textit{ soft, foamy substance in a pressurized canister.}

\noindent
\textbf{shawl:}\textit{ large, rectangular or triangular piece of fabric draped over the shoulders.}

\noindent
\textbf{shears:}\textit{ large scissors with long blades, used for cutting thick materials.}

\noindent
\textbf{sheep:}\textit{ woolly animal with a round body and a gentle face.}

\noindent
\textbf{shepherd\_dog:}\textit{ medium-sized, furry dog with pointed ears and a long snout.}

\noindent
\textbf{sherbert:}\textit{ soft, smooth, brightly colored frozen dessert.}

\noindent
\textbf{shield:}\textit{ large, round or rectangular piece of metal or wood, often with a handle.}

\noindent
\textbf{shirt:}\textit{ soft, collared or uncollared garment with buttons and sleeves.}

\noindent
\textbf{shoe:}\textit{ footwear with a solid sole and an enclosed upper.}

\noindent
\textbf{shopping\_bag:}\textit{ large, rectangular bag with handles, made of paper or plastic.}

\noindent
\textbf{shopping\_cart:}\textit{ metal or plastic basket on wheels with a handle.}

\noindent
\textbf{short\_pants:}\textit{ knee-length pants with a waistband and pockets.}

\noindent
\textbf{shot\_glass:}\textit{ small, cylindrical glass with thick sides, used for serving drinks.}

\noindent
\textbf{shoulder\_bag:}\textit{ soft, rectangular bag with a long strap, worn over the shoulder.}

\noindent
\textbf{shovel:}\textit{ long-handled tool with a wide, flat metal blade for digging.}

\noindent
\textbf{shower\_head:}\textit{ circular or square device with holes, attached to a water pipe.}

\noindent
\textbf{shower\_cap:}\textit{ waterproof, elastic banded cover for the head.}

\noindent
\textbf{shower\_curtain:}\textit{ large, rectangular piece of fabric or plastic hung to block water.}

\noindent
\textbf{shredder\_(for\_paper):}\textit{ rectangular box with slots for inserting paper, often with blades inside.}

\noindent
\textbf{signboard:}\textit{ flat, rectangular or square board with writing or symbols.}

\noindent
\textbf{silo:}\textit{ tall, cylindrical structure, often with a domed top, for storing grain.}

\noindent
\textbf{sink:}\textit{ shallow basin with a faucet and drain, typically made of metal or porcelain.}

\noindent
\textbf{skateboard:}\textit{ flat, narrow board with four wheels and upward-curved ends.}

\noindent
\textbf{skewer:}\textit{ thin, sharp metal or wooden stick for grilling food.}

\noindent
\textbf{ski:}\textit{ long, narrow board with a slightly curved tip, worn on the feet for sliding on snow.}

\noindent
\textbf{ski\_boot:}\textit{ stiff, high-ankle boot with clips or straps for attaching to skis.}

\noindent
\textbf{ski\_parka:}\textit{ thick, padded jacket with a hood, designed for cold weather.}

\noindent
\textbf{ski\_pole:}\textit{ thin, metal rod with a handle and a small disc near the base.}

\noindent
\textbf{skirt:}\textit{ soft, flowy garment that wraps around the waist and falls to the legs.}

\noindent
\textbf{skullcap:}\textit{ small, tight-fitting cap worn on the head.}

\noindent
\textbf{sled:}\textit{ flat, narrow platform with runners for sliding over snow.}

\noindent
\textbf{sleeping\_bag:}\textit{ long, padded fabric bag with a zipper, used for sleeping.}

\noindent
\textbf{sling\_(bandage):}\textit{ soft, triangular or rectangular fabric strap for supporting an arm.}

\noindent
\textbf{slipper\_(footwear):}\textit{ soft, low-cut shoe with an open or closed heel.}

\noindent
\textbf{smoothie:}\textit{ thick, colorful drink in a glass or bottle, often with fruit on top.}

\noindent
\textbf{snake:}\textit{ long, slender, scaly reptile with a pointed head and a flicking tongue.}

\noindent
\textbf{snowboard:}\textit{ flat, wide board with a slightly upturned front, used for sliding on snow.}

\noindent
\textbf{snowman:}\textit{ rounded figure made of stacked snowballs, often with a scarf and hat.}

\noindent
\textbf{snowmobile:}\textit{ low, motorized vehicle with tracks or skis for traveling on snow.}

\noindent
\textbf{soap:}\textit{ small, rectangular or oval block of solid cleaning substance.}

\noindent
\textbf{soccer\_ball:}\textit{ round, black and white paneled ball.}

\noindent
\textbf{sock:}\textit{ soft, tubular fabric worn on the foot.}

\noindent
\textbf{sofa:}\textit{ large, cushioned seat with a backrest and armrests.}

\noindent
\textbf{softball:}\textit{ round ball, slightly larger than a baseball, with visible stitching.}

\noindent
\textbf{solar\_array:}\textit{ flat, rectangular panels with a shiny, grid-like surface.}

\noindent
\textbf{sombrero:}\textit{ large, round hat with a wide, floppy brim and a high crown.}

\noindent
\textbf{soup:}\textit{ liquid meal in a bowl, often with visible ingredients like vegetables or noodles.}

\noindent
\textbf{soup\_bowl:}\textit{ deep, round bowl with a wide rim, often ceramic.}

\noindent
\textbf{soupspoon:}\textit{ round, shallow spoon with a wide bowl.}

\noindent
\textbf{sour\_cream:}\textit{ soft, thick, white dairy product in a small bowl or tub.}

\noindent
\textbf{soya\_milk:}\textit{ pale, creamy liquid in a glass or carton.}

\noindent
\textbf{space\_shuttle:}\textit{ large, sleek, winged spacecraft with a pointed nose.}

\noindent
\textbf{sparkler\_(fireworks):}\textit{ thin metal stick that produces bright, sparkling light when lit.}

\noindent
\textbf{spatula:}\textit{ flat, wide tool with a handle, often used for flipping food.}

\noindent
\textbf{spear:}\textit{ long, straight pole with a pointed tip, often metal.}

\noindent
\textbf{spectacles:}\textit{ thin, wire or plastic frame with two round or rectangular lenses.}

\noindent
\textbf{spice\_rack:}\textit{ small, rectangular shelf with jars or bottles of spices.}

\noindent
\textbf{spider:}\textit{ small, eight-legged creature with a round body and segmented legs.}

\noindent
\textbf{crawfish:}\textit{ small, lobster-like crustacean with a hard shell and long claws.}

\noindent
\textbf{sponge:}\textit{ soft, porous material, often rectangular or oval, used for cleaning.}

\noindent
\textbf{spoon:}\textit{ small, curved utensil with a long handle and a round, shallow bowl.}

\noindent
\textbf{sportswear:}\textit{ colorful athletic clothing for exercise.}

\noindent
\textbf{spotlight:}\textit{ round, bright light used for illumination.}

\noindent
\textbf{squid\_(food):}\textit{ soft, often translucent, sea creature.}

\noindent
\textbf{squirrel:}\textit{ small, furry rodent with a bushy tail.}

\noindent
\textbf{stagecoach:}\textit{ wooden carriage on wheels, often vintage.}

\noindent
\textbf{stapler\_(stapling\_machine):}\textit{ metal and plastic device for fastening papers.}

\noindent
\textbf{starfish:}\textit{ star-shaped marine animal with five arms.}

\noindent
\textbf{statue\_(sculpture):}\textit{ three-dimensional sculpture made of stone or metal.}

\noindent
\textbf{steak\_(food):}\textit{ thick cut of meat, usually red or brown.}

\noindent
\textbf{steak\_knife:}\textit{ sharp, serrated knife with a smooth handle.}

\noindent
\textbf{steering\_wheel:}\textit{ round wheel for controlling a vehicle.}

\noindent
\textbf{stepladder:}\textit{ foldable ladder with steps for reaching heights.}

\noindent
\textbf{step\_stool:}\textit{ small stool for standing on to reach higher places.}

\noindent
\textbf{stereo\_(sound\_system):}\textit{ boxy audio system with speakers.}

\noindent
\textbf{stew:}\textit{ thick, hearty mixture of ingredients in a bowl.}

\noindent
\textbf{stirrer:}\textit{ long utensil used for mixing liquids.}

\noindent
\textbf{stirrup:}\textit{ curved support for a rider’s foot on a saddle.}

\noindent
\textbf{stool:}\textit{ short, simple seat without a backrest.}

\noindent
\textbf{stop\_sign:}\textit{ red, octagonal sign indicating to halt.}

\noindent
\textbf{brake\_light:}\textit{ red light on vehicles that indicates stopping.}

\noindent
\textbf{stove:}\textit{ flat surface appliance for cooking food.}

\noindent
\textbf{strainer:}\textit{ bowl-shaped tool with holes for draining liquids.}

\noindent
\textbf{strap:}\textit{ long, narrow band for securing or holding.}

\noindent
\textbf{straw\_(for\_drinking):}\textit{ thin tube for sipping liquids.}

\noindent
\textbf{strawberry:}\textit{ red, heart-shaped fruit with tiny seeds.}

\noindent
\textbf{street\_sign:}\textit{ rectangular sign displaying road information.}

\noindent
\textbf{streetlight:}\textit{ tall pole with a light for illuminating roads.}

\noindent
\textbf{string\_cheese:}\textit{ soft cheese in long, thin strands.}

\noindent
\textbf{stylus:}\textit{ thin pen-like tool for touchscreen devices.}

\noindent
\textbf{subwoofer:}\textit{ large speaker for deep bass sounds.}

\noindent
\textbf{sugar\_bowl:}\textit{ small container for holding sugar.}

\noindent
\textbf{sugarcane\_(plant):}\textit{ tall plant with thick, jointed stems.}

\noindent
\textbf{suit\_(clothing):}\textit{ formal clothing consisting of a jacket and trousers.}

\noindent
\textbf{sunflower:}\textit{ tall plant with a large yellow flower head.}

\noindent
\textbf{sunglasses:}\textit{ dark glasses for protecting eyes from sunlight.}

\noindent
\textbf{sunhat:}\textit{ wide-brimmed hat for shading the face.}

\noindent
\textbf{surfboard:}\textit{ long, flat board for riding ocean waves.}

\noindent
\textbf{sushi:}\textit{ small rolls of rice and seafood, often colorful.}

\noindent
\textbf{mop:}\textit{ long-handled tool with a cloth head for cleaning.}

\noindent
\textbf{sweat\_pants:}\textit{ loose-fitting pants for comfort and exercise.}

\noindent
\textbf{sweatband:}\textit{ cloth band worn on the forehead during sports.}

\noindent
\textbf{sweater:}\textit{ knitted garment worn on the upper body.}

\noindent
\textbf{sweatshirt:}\textit{ pullover top made of thick, soft fabric.}

\noindent
\textbf{sweet\_potato:}\textit{ orange, starchy tuber with a smooth skin.}

\noindent
\textbf{swimsuit:}\textit{ tight-fitting clothing for swimming.}

\noindent
\textbf{sword:}\textit{ long, sharp weapon with a straight blade.}

\noindent
\textbf{syringe:}\textit{ cylindrical tube used for injecting liquids.}

\noindent
\textbf{tabasco\_sauce:}\textit{ small bottle containing spicy pepper sauce.}

\noindent
\textbf{table-tennis\_table:}\textit{ rectangular surface for playing table tennis.}

\noindent
\textbf{table:}\textit{ flat surface supported by legs.}

\noindent
\textbf{table\_lamp:}\textit{ small lamp with a base for tables.}

\noindent
\textbf{tablecloth:}\textit{ fabric cover for protecting a table.}

\noindent
\textbf{tachometer:}\textit{ gauge measuring engine speed, often circular.}

\noindent
\textbf{taco:}\textit{ folded tortilla filled with various ingredients.}

\noindent
\textbf{tag:}\textit{ small label attached to an item for identification.}

\noindent
\textbf{taillight:}\textit{ red light at the back of vehicles.}

\noindent
\textbf{tambourine:}\textit{ circular instrument with jingles around the edge.}

\noindent
\textbf{army\_tank:}\textit{ armored vehicle with a rotating turret.}

\noindent
\textbf{tank\_(storage\_vessel):}\textit{ large container for holding liquids.}

\noindent
\textbf{tank\_top\_(clothing):}\textit{ sleeveless shirt often worn casually.}

\noindent
\textbf{tape\_(sticky\_cloth\_or\_paper):}\textit{ flexible strip for sticking items together.}

\noindent
\textbf{tape\_measure:}\textit{ flexible ruler for measuring lengths.}

\noindent
\textbf{tapestry:}\textit{ decorative fabric with intricate designs.}

\noindent
\textbf{tarp:}\textit{ large, waterproof cover, often made of plastic.}

\noindent
\textbf{tartan:}\textit{ pattern of crisscrossed horizontal and vertical bands.}

\noindent
\textbf{tassel:}\textit{ decorative hanging made of threads or strands.}

\noindent
\textbf{tea\_bag:}\textit{ small pouch containing tea leaves.}

\noindent
\textbf{teacup:}\textit{ small cup used for drinking tea.}

\noindent
\textbf{teakettle:}\textit{ metal pot with a spout for boiling water.}

\noindent
\textbf{teapot:}\textit{ container for brewing and serving tea.}

\noindent
\textbf{teddy\_bear:}\textit{ soft, stuffed toy bear.}

\noindent
\textbf{telephone:}\textit{ device for voice communication.}

\noindent
\textbf{telephone\_booth:}\textit{ small enclosure for making phone calls.}

\noindent
\textbf{telephone\_pole:}\textit{ tall post for holding telephone wires.}

\noindent
\textbf{telephoto\_lens:}\textit{ long camera lens for distant subjects.}

\noindent
\textbf{television\_camera:}\textit{ device for capturing moving images.}

\noindent
\textbf{television\_set:}\textit{ boxy device for displaying video content.}

\noindent
\textbf{tennis\_ball:}\textit{ yellow, fuzzy ball used in tennis.}

\noindent
\textbf{tennis\_racket:}\textit{ long handle with a netted head for hitting balls.}

\noindent
\textbf{tequila:}\textit{ clear, alcoholic beverage in a bottle.}

\noindent
\textbf{thermometer:}\textit{ instrument for measuring temperature.}

\noindent
\textbf{thermos\_bottle:}\textit{ insulated container for keeping liquids hot or cold.}

\noindent
\textbf{thermostat:}\textit{ device for regulating temperature.}

\noindent
\textbf{thimble:}\textit{ small protective cap for sewing fingers.}

\noindent
\textbf{thread:}\textit{ thin strand used for sewing.}

\noindent
\textbf{thumbtack:}\textit{ small pin for attaching papers to surfaces.}

\noindent
\textbf{tiara:}\textit{ ornate crown worn on the head.}

\noindent
\textbf{tiger:}\textit{ large striped cat with orange and black fur.}

\noindent
\textbf{tights\_(clothing):}\textit{ close-fitting legwear made of stretchy fabric.}

\noindent
\textbf{timer:}\textit{ device for measuring time intervals.}

\noindent
\textbf{tinfoil:}\textit{ thin, shiny metal sheet used for wrapping.}

\noindent
\textbf{tinsel:}\textit{ shiny strands used for decoration.}

\noindent
\textbf{tissue\_paper:}\textit{ soft, thin paper often used for wrapping.}

\noindent
\textbf{toast\_(food):}\textit{ browned slice of bread.}

\noindent
\textbf{toaster:}\textit{ appliance for browning bread slices.}

\noindent
\textbf{toaster\_oven:}\textit{ small oven for toasting and baking.}

\noindent
\textbf{toilet:}\textit{ ceramic fixture for waste disposal.}

\noindent
\textbf{toilet\_tissue:}\textit{ soft paper for personal hygiene.}

\noindent
\textbf{tomato:}\textit{ round, red fruit with a smooth skin.}

\noindent
\textbf{tongs:}\textit{ pincers used for gripping food.}

\noindent
\textbf{toolbox:}\textit{ box for storing tools, often metal or plastic.}

\noindent
\textbf{toothbrush:}\textit{ small brush for cleaning teeth.}

\noindent
\textbf{toothpaste:}\textit{ cream used with a toothbrush for cleaning teeth.}

\noindent
\textbf{toothpick:}\textit{ small stick for cleaning between teeth.}

\noindent
\textbf{cover:}\textit{ material used to protect or enclose something.}

\noindent
\textbf{tortilla:}\textit{ flat, round bread made from corn or wheat.}

\noindent
\textbf{tow\_truck:}\textit{ vehicle designed for pulling other vehicles.}

\noindent
\textbf{towel:}\textit{ absorbent cloth for drying hands or body.}

\noindent
\textbf{towel\_rack:}\textit{ bar for hanging towels.}

\noindent
\textbf{toy:}\textit{ object for play, often colorful and fun.}

\noindent
\textbf{tractor\_(farm\_equipment):}\textit{ large vehicle for farming tasks.}

\noindent
\textbf{traffic\_light:}\textit{ signal with red, yellow, and green lights.}

\noindent
\textbf{dirt\_bike:}\textit{ small motorcycle designed for off-road riding.}

\noindent
\textbf{trailer\_truck:}\textit{ large vehicle for transporting goods.}

\noindent
\textbf{train\_(railroad\_vehicle):}\textit{ long vehicle on tracks for transporting people or goods.}

\noindent
\textbf{trampoline:}\textit{ bouncy surface for jumping.}

\noindent
\textbf{tray:}\textit{ flat surface for carrying items.}

\noindent
\textbf{trench\_coat:}\textit{ long, waterproof coat for protection.}

\noindent
\textbf{triangle\_(musical\_instrument):}\textit{ three-sided musical instrument.}

\noindent
\textbf{tricycle:}\textit{ three-wheeled bicycle for children.}

\noindent
\textbf{tripod:}\textit{ stand with three legs for stabilizing cameras.}

\noindent
\textbf{trousers:}\textit{ long pants for clothing.}

\noindent
\textbf{truck:}\textit{ large vehicle for transporting goods.}

\noindent
\textbf{truffle\_(chocolate):}\textit{ rich chocolate confection, often round.}

\noindent
\textbf{trunk:}\textit{ large, sturdy container for storage.}

\noindent
\textbf{vat:}\textit{ large container for holding liquids.}

\noindent
\textbf{turban:}\textit{ cloth wrapped around the head.}

\noindent
\textbf{turkey\_(food):}\textit{ large bird, often cooked for holidays.}

\noindent
\textbf{turnip:}\textit{ round, edible root vegetable.}

\noindent
\textbf{turtle:}\textit{ reptile with a hard shell.}

\noindent
\textbf{turtleneck\_(clothing):}\textit{ close-fitting sweater with a high collar.}

\noindent
\textbf{typewriter:}\textit{ mechanical device for typing letters.}

\noindent
\textbf{umbrella:}\textit{ portable cover for protection from rain.}

\noindent
\textbf{underwear:}\textit{ garments worn beneath outer clothing.}

\noindent
\textbf{unicycle:}\textit{ one-wheeled bicycle for balance.}

\noindent
\textbf{urinal:}\textit{ fixture for urinating, usually in restrooms.}

\noindent
\textbf{urn:}\textit{ decorative container for holding ashes or flowers.}

\noindent
\textbf{vacuum\_cleaner:}\textit{ device for cleaning floors using suction.}

\noindent
\textbf{vase:}\textit{ container for holding flowers.}

\noindent
\textbf{vending\_machine:}\textit{ automated machine for selling snacks or drinks.}

\noindent
\textbf{vent:}\textit{ opening for air circulation.}

\noindent
\textbf{vest:}\textit{ sleeveless garment worn over a shirt.}

\noindent
\textbf{videotape:}\textit{ magnetic tape for recording video.}

\noindent
\textbf{vinegar:}\textit{ sour liquid used in cooking and dressing.}

\noindent
\textbf{violin:}\textit{ string instrument played with a bow.}

\noindent
\textbf{vodka:}\textit{ clear, distilled alcoholic beverage.}

\noindent
\textbf{volleyball:}\textit{ light ball used in the sport of volleyball.}

\noindent
\textbf{vulture:}\textit{ large bird often seen scavenging.}

\noindent
\textbf{waffle:}\textit{ light, crispy batter cooked in a patterned iron.}

\noindent
\textbf{waffle\_iron:}\textit{ device for cooking waffles.}

\noindent
\textbf{wagon:}\textit{ four-wheeled vehicle for transporting items.}

\noindent
\textbf{wagon\_wheel:}\textit{ round wooden or metal wheel for wagons.}

\noindent
\textbf{walking\_stick:}\textit{ long stick used for support while walking.}

\noindent
\textbf{wall\_clock:}\textit{ clock mounted on a wall.}

\noindent
\textbf{wall\_socket:}\textit{ electrical outlet for plugging in devices.}

\noindent
\textbf{wallet:}\textit{ small, foldable case for holding money and cards.}

\noindent
\textbf{walrus:}\textit{ large marine mammal with tusks.}

\noindent
\textbf{wardrobe:}\textit{ tall cabinet for storing clothes.}

\noindent
\textbf{washbasin:}\textit{ bowl for washing hands or face.}

\noindent
\textbf{automatic\_washer:}\textit{ appliance for cleaning clothes.}

\noindent
\textbf{watch:}\textit{ small timekeeping device worn on the wrist.}

\noindent
\textbf{water\_bottle:}\textit{ container for holding drinking water.}

\noindent
\textbf{water\_cooler:}\textit{ appliance for dispensing chilled water.}

\noindent
\textbf{water\_faucet:}\textit{ tap for controlling water flow.}

\noindent
\textbf{water\_heater:}\textit{ device for heating water.}

\noindent
\textbf{water\_jug:}\textit{ large container for holding water.}

\noindent
\textbf{water\_gun:}\textit{ toy for spraying water.}

\noindent
\textbf{water\_scooter:}\textit{ small vehicle for riding on water.}

\noindent
\textbf{water\_ski:}\textit{ equipment for skiing on water.}

\noindent
\textbf{water\_tower:}\textit{ tall structure for storing water.}

\noindent
\textbf{watering\_can:}\textit{ container with a spout for watering plants.}

\noindent
\textbf{watermelon:}\textit{ large, green fruit with sweet, red flesh.}

\noindent
\textbf{weathervane:}\textit{ device showing wind direction, often decorative.}

\noindent
\textbf{webcam:}\textit{ camera used for video streaming.}

\noindent
\textbf{wedding\_cake:}\textit{ decorative cake served at weddings.}

\noindent
\textbf{wedding\_ring:}\textit{ circular band worn during marriage.}

\noindent
\textbf{wet\_suit:}\textit{ tight-fitting suit for water activities.}

\noindent
\textbf{wheel:}\textit{ circular object for movement.}

\noindent
\textbf{wheelchair:}\textit{ chair with wheels for mobility.}

\noindent
\textbf{whipped\_cream:}\textit{ light, fluffy cream used as a topping.}

\noindent
\textbf{whistle:}\textit{ small device that makes a high-pitched sound.}

\noindent
\textbf{wig:}\textit{ artificial hairpiece worn on the head.}

\noindent
\textbf{wind\_chime:}\textit{ decorative item that makes sound in the wind.}

\noindent
\textbf{windmill:}\textit{ structure for harnessing wind energy.}

\noindent
\textbf{window\_box\_(for\_plants):}\textit{ container for growing plants outside windows.}

\noindent
\textbf{windshield\_wiper:}\textit{ device for clearing rain from windshields.}

\noindent
\textbf{windsock:}\textit{ fabric cone indicating wind direction.}

\noindent
\textbf{wine\_bottle:}\textit{ bottle for storing wine.}

\noindent
\textbf{wine\_bucket:}\textit{ container for chilling wine bottles.}

\noindent
\textbf{wineglass:}\textit{ stemmed glass for drinking wine.}

\noindent
\textbf{blinder\_(for\_horses):}\textit{ covers for horses’ eyes to reduce distractions.}

\noindent
\textbf{wok:}\textit{ deep, round pan used for stir-frying.}

\noindent
\textbf{wolf:}\textit{ wild canine known for its pack behavior.}

\noindent
\textbf{wooden\_spoon:}\textit{ kitchen tool for stirring.}

\noindent
\textbf{wreath:}\textit{ circular decoration, often made of leaves or flowers.}

\noindent
\textbf{wrench:}\textit{ tool for gripping and turning nuts and bolts.}

\noindent
\textbf{wristband:}\textit{ band worn around the wrist, often for events.}

\noindent
\textbf{wristlet:}\textit{ small pouch with a strap for carrying.}

\noindent
\textbf{yacht:}\textit{ luxury boat for recreation.}

\noindent
\textbf{yogurt:}\textit{ creamy dairy product, often flavored.}

\noindent
\textbf{yoke\_(animal\_equipment):}\textit{ wooden beam for joining animals together.}

\noindent
\textbf{zebra:}\textit{ striped black and white animal.}

\noindent
\textbf{zucchini:}\textit{ long, green vegetable, often used in cooking.}
